# Supplementary material for: Circuit Depth Reduction for Executable Hamiltonian Dynamics of Covalent Inhibitor Reactivity on Quantum Hardware
Source: arXiv:2412.15804 source file (2026-08-28)
Supplement: Supplementary file 1 [file supplementary_information.tex]

\documentclass[pra,preprint]{revtex4-2}

\usepackage{graphicx}
\usepackage{caption}
\usepackage{placeins}
\usepackage{hyperref}
\usepackage{subcaption}
\usepackage{enumitem}% http://ctan.org/pkg/enumitem
\usepackage[title]{appendix}
\usepackage{algorithm}
\usepackage{algpseudocode}

\usepackage{amsmath}

\begin{document}

\newcommand{\sulf}{SO\textsubscript{2}F} %for sulfonyl fluoride formula

\title{Efficient Hamiltonian Simulation: A Utility Scale Perspective for Covalent Inhibitor Reactivity Prediction}
\author{Marek Kowalik$^1$, Sam Genway$^1$, Vedangi Pathak$^{2, 3}$, Mykola Maksymenko$^4$, Simon Martiel$^{5}$, Hamed Mohammadbagherpoor$^{2}$, Richard Padbury$^{2}$, Vladyslav Los$^{4,6}$, Oleksa Hryniv$^4$, Peter Pog\'{a}ny$^7$, Phalgun Lolur$^{1*}$}
\maketitle

\par{$^1$ Capgemini Quantum Lab}
\par{$^2$ IBM T. J. Watson Research Center, Yorktown Heights, NY}
\par{$^3$ Department of Physics and Astronomy at University of British Columbia}
\par{$^4$ Haiqu Inc.}
\par{$^5$ IBM Quantum, IBM France Lab, Orsay, France}
\par{$^6$ Institute for Quantum Information, RWTH Aachen University}
\par{$^7$ GSK Medicines Research Centre, Gunnels Wood Road, Stevenage,
Hertfordshire SG1 2NY, United Kingdom}
\par{$^*$ Corresponding author - phalgun.lolur@capgemini.com}

\newpage

\section{Quantum Chemistry Simulations on Quantum Computers}
\label{SI_subsec:quantum chemistry sim on quantum computers}

The starting point for Hamiltonian simulation is the electronic structure Hamiltonian. Specifically, we use the Fermionic Hamiltonian in the second quantized form:
$$ 
\hat{H}_f=\ \sum_{ij}^{M}{h_{ij}{\hat{a}}_i^\dagger{\hat{a}}_j+\sum_{ijkl}^{M}{h_{ijkl}{\hat{a}}_i^\dagger{\hat{a}}_j^\dagger{\hat{a}}_k{\hat{a}}_l}}
$$
where the summation is performed over the active space size, with $h_{ij}$ and $h_{ijkl}$ representing the one- and two-electron integrals of the operators projected into a given basis set, respectively. The ${\hat{a}}_i^\dagger$ and ${\hat{a}}_i$ are fermionic creation and annihilation operators, respectively. 
To perform Hamiltonian simulations using quantum computers, any given Hamiltonian needs to be converted to a suitable fermionic-to-qubit mapping given as follows:
$$
\hat{H}_q=\ \sum_{k=1}^{K}{c_k{\hat{P}}_k}
$$ 
where $c_k$ denotes the coefficient, and ${\hat{P}}_k$ are the tensor products of Pauli matrices, further called ‘Pauli strings’ (or ‘Pauli words’), acting on N qubits:
$$
{\hat{P}}_k=\ {\hat{p}}_{1k}\ \otimes\ {\hat{p}}_{1k}\otimes\ldots\ \otimes\ {\hat{p}}_{Nk}
$$
where ${\hat{p}}_{1k}\in\left\{I,{\hat{\sigma}}_x,\ {\hat{\sigma}}_y,\ {\hat{\sigma}}_z\right\}$, with $I$ denoting identity matrix, and $\hat{\sigma_i}$ representing the Pauli matrices. To shorten descriptions, a more efficient notation is often used with just the letters $X$, $Y$, $Z$, and $I$ with omitted tensor product signs. There are various qubit mapping methods for chemistry problems such as Jordan-Wigner or Bravyi–Kitaev and alternative methods that consider device connectivity such as the Bonsai algorithm\cite{Miller2023}. It is important to note that efficient fermionic-to-qubit mappings are also key to achieving shallower circuits, as efficient mappings not only consider the structure of the problem but also factor in the connectivity of the QPU architecture. This work focuses on simulating the time evolution of a given observable of the chosen system. Quantum computing is utilized to simulate the time-evolved state of the system to a given point in time and to finally measure the expectation value with the appropriate measurement operator. By choosing the Schrödinger representation, the evolved state $\psi(t)$ can be calculated by operating the initial state at time $t_0=0$ with the time evolution operator $\hat{U}(t)$ as given by:
$$|\psi(t)\rangle=\hat{U}(t)|\psi(t_0)\rangle $$
where:
$$
\hat{U}(t)=e^{-i\hat{H}t}\ 
$$
The evolution operator above in exponent form is one of the possible solutions of the time-dependent Schrödinger equation. Finally, the observable of choice for the system needs to be prepared as a measurement operator $\hat{O}$ in the qubit mapped form. To recreate the time evolution curve of the given observable, its expectation value needs to be estimated over different times $t$:
$$
\langle\psi(t) | \hat{O} | \psi(t)\rangle
$$
In the simplest case of energy time evolution, the observable is the same qubit-mapped Hamiltonian used in the time evolution operator. Other observables can be defined to more effectively predict molecule reactivity \cite{Montgomery2023}. In this paper, we leverage the product formulas (PF) decomposition\cite{Berry2006} to implement real-time quantum system evolution as described in Section~SI~\ref{SI_sec:product_formulas}.

\newpage
\section{Product Formulas}
\label{SI_sec:product_formulas}

The most straightforward method to simulate real-time evolution of quantum systems is to encode the initial state of the simulated system into qubit states (using the same qubit mapping scheme as for the transformation of Hamiltonian from fermionic to qubit mapped form) and evolve them with the time evolution operator as the direct exponentiation of Hamiltonian terms using PF approximations, also called Trotter formulas or Trotter-Suzuki decompositions. This way, to recreate the observable trajectory, a series of subexperiments is conducted to estimate the expectation value at a set of time points. In each subexperiment the initial state is encoded, then the time evolution operator is applied to transform the state to a given time point, and finally, the observable expectation value is measured. A high-level scheme of such subexperiment's quantum circuit is shown in Figure \ref{fig:time evolution simulation circuit scheme}. 

\vspace{\baselineskip}
\begin{figure}[h]
    \begin{minipage}{\linewidth}
        \centering
        \resizebox{0.9\linewidth}{!}{\includegraphics{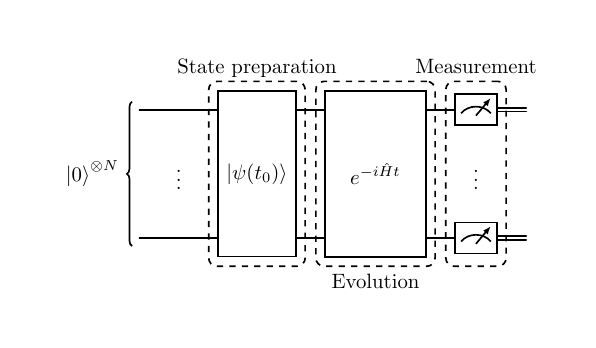}}
    \end{minipage}
    \caption{\textit{Scheme of the real-time evolution simulation circuit}}
    \label{fig:time evolution simulation circuit scheme}
\end{figure}

The challenge lies in the effective and accurate preparation of the time evolution operator. The Product Formulas are the way to approximate the operator so that it can be applied on QPUs. In general, terms in the qubit mapped Hamiltonian $\hat{H}_q$ do not commute, which means, that the time evolution operator cannot be prepared as a product of operators of each Pauli term:
$$
e^{-i\hat{H}_qt}=e^{-i(c_1{\hat{P}}_1+\ \ldots\ {+\ c}_k{\hat{P}}_k)t}\neq e^{-i(c_1{\hat{P}}_1)t}{\ldots e}^{-i(c_k{\hat{P}}_k)t}
$$
The most straightforward approximation is the first-order PF, called Lie-Trotter product formula:
$$
e^{-i(c_1{\hat{P}}_1+\ \ldots\ {+\ c}_k{\hat{P}}_k)t} = \lim_{n\rightarrow\infty}{\left(e^\frac{-i\left(c_1{\hat{P}}_1\right)t}{n}\ {\ \ldots e}^\frac{-i\left(c_k{\hat{P}}_k\right)t}{n}\right)^n}
$$
Where \textit{n}, the so-called Trotter number or number of Trotter steps, is an arbitrary number adjusting the level of approximation for the physical implementation on QPUs. 

\vspace{\baselineskip}
\begin{figure}[h]
    \begin{minipage}{\linewidth}
        \centering
        \resizebox{0.95\linewidth}{!}{\includegraphics{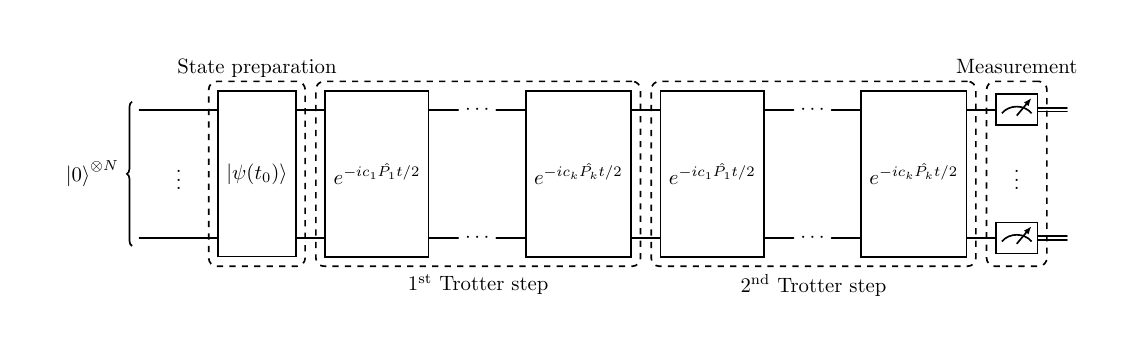}}
        \end{minipage}
    \caption{\textit{Time evolution simulation circuit approximated with two Trotter steps}}
    \label{fig:time evolution simulation circuit 2 trotter steps}
\end{figure}

Higher-order formulas were proposed to decompose exponent with the sum of terms more efficiently, that means with a faster decrease in error with a number of Trotter steps so that the shallower circuit can be made to express the same problem with the same accuracy or the circuit of the similar depth with better accuracy than the one obtained from lower-order formulas. A good overview of those is in \cite{Ostmeyer2023}. 

\newpage
\section{Pauli Strings Exponentiation gate cost}
\label{SI_sec:pauli_strings_exponentation_gate_cost}

To understand the gate complexity of the circuits produced by PFs, the application of each exponentiated Pauli term operator on the quantum circuit needs to be considered. Each arbitrary term can be applied exactly on a gate-based quantum computer.

For instance, let us take the term $\hat{P}=\ {\hat{\sigma}}_z\otimes\hat{I}\otimes{\hat{\sigma}}_x\otimes{\hat{\sigma}}_y\otimes{\hat{\sigma}}_z$, with some coefficient $c_i$. First, the term is diagonalized by changing the basis to the computational one, on the qubits, where ${\hat{\sigma}}_x$ and ${\hat{\sigma}}_y$ are applied. Now, all the qubits influenced by the term (i.e. with respective non-identity matrix in the term) are ready to apply the term in the computational basis. Then the parity check is performed, since for terms with computational basis vectors, the eigenvalues are determined by the parity of the vector bit strings. The parity check can be done efficiently on QPU with linear connectivity with the ‘chain’ or ‘ladder’ of CNOTs, as shown in Figure \ref{fig:Pauli term exp. on circuit example}. Then a single $R_z$ rotation is applied depending on the simulated time step and the term coefficient. The circuit is finalized with the parity check uncomputing and changing back the basis of qubits.
\vspace{\baselineskip}
\begin{figure}[h]
    \begin{minipage}{\linewidth}
        \centering
        \resizebox{0.95\linewidth}{!}{\includegraphics{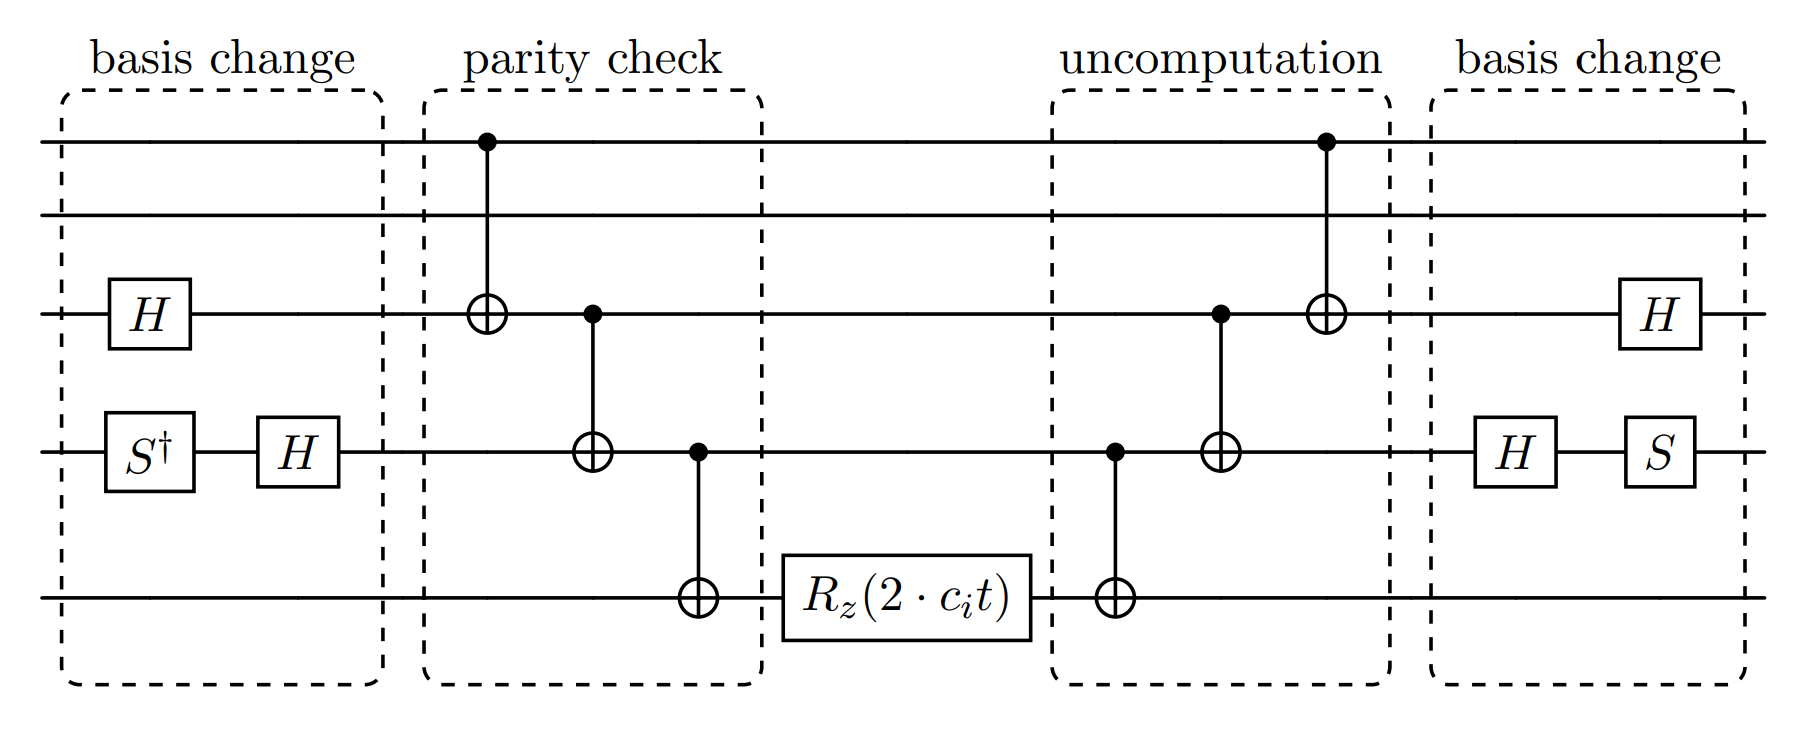}}
        \end{minipage}
    \caption{\textit{Example of Pauli string ${\hat{\sigma}}_z\otimes\hat{I}\otimes{\hat{\sigma}}_x \otimes{\hat{\sigma}}_y\otimes{\hat{\sigma}}_z$ ($ZIXYZ$) exponentiation on a quantum circuit.}}
    \label{fig:Pauli term exp. on circuit example}
\end{figure}

This gives a way to express the exponentiated Pauli terms of a weight w with $2(w-1)$ CNOT gates and maximally $4w+1$ single qubit gates. Now, let us consider the real backend case. To make it general, let us consider a backend with linear connectivity and $Clifford+R_z$ basis gate set. Each of the identity operators in the Pauli term, which has a non-identity operator before or after itself, requires 2 swap gates, which in general requires 3 CNOT gates to decompose each as shown in Figure \ref{fig:Pauli term exp. on circuit with ID terms example}.

\vspace{\baselineskip}
\begin{figure}[h]
    \begin{minipage}{\linewidth}
        \centering
        \resizebox{0.95\linewidth}{!}{\includegraphics[]{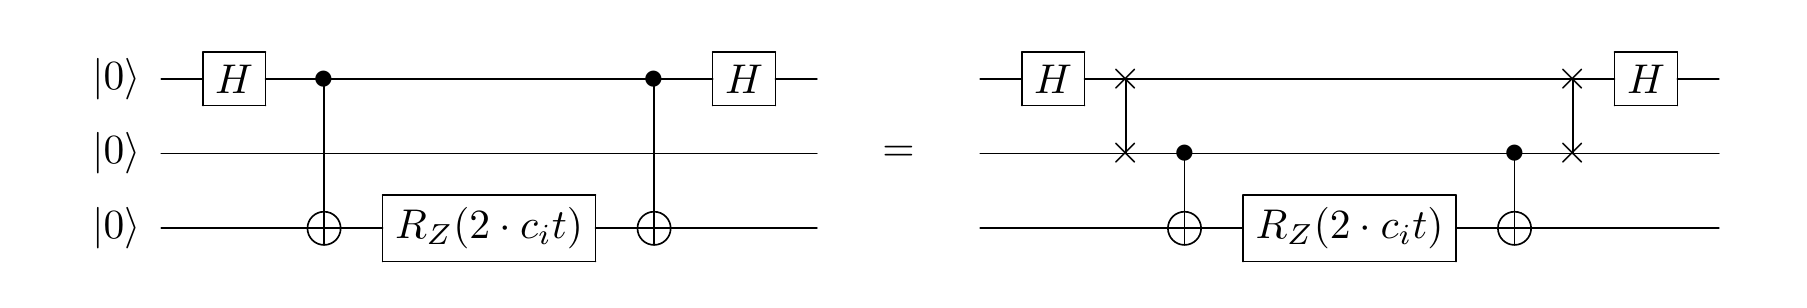}}
        \resizebox{0.95\linewidth}{!}{\includegraphics[]{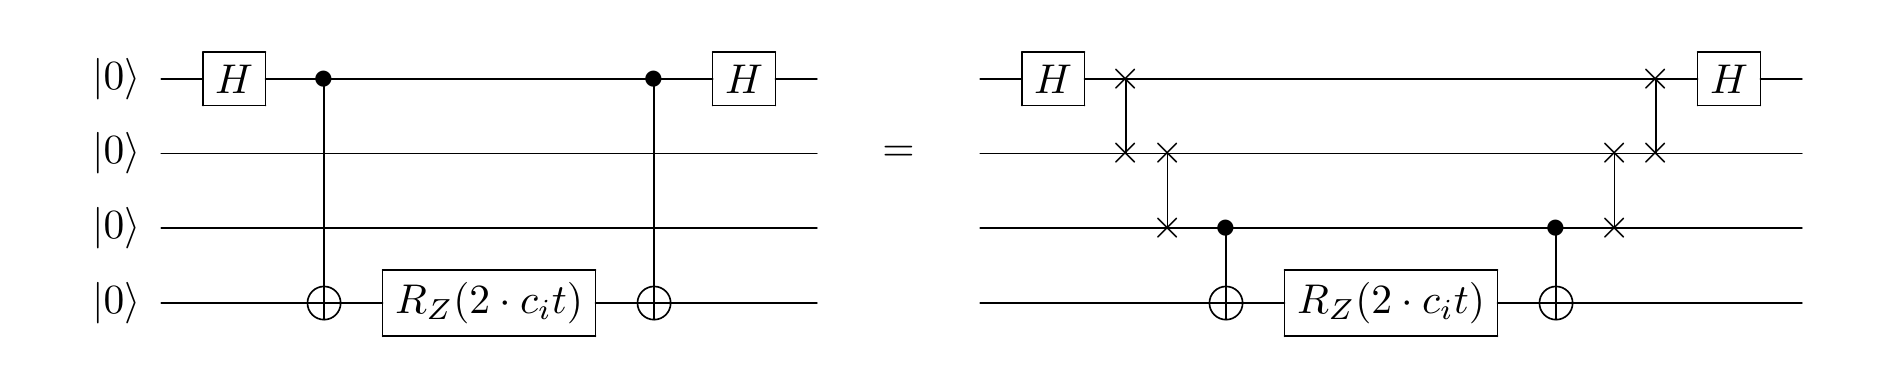}}
        \resizebox{0.95\linewidth}{!}{\includegraphics[]{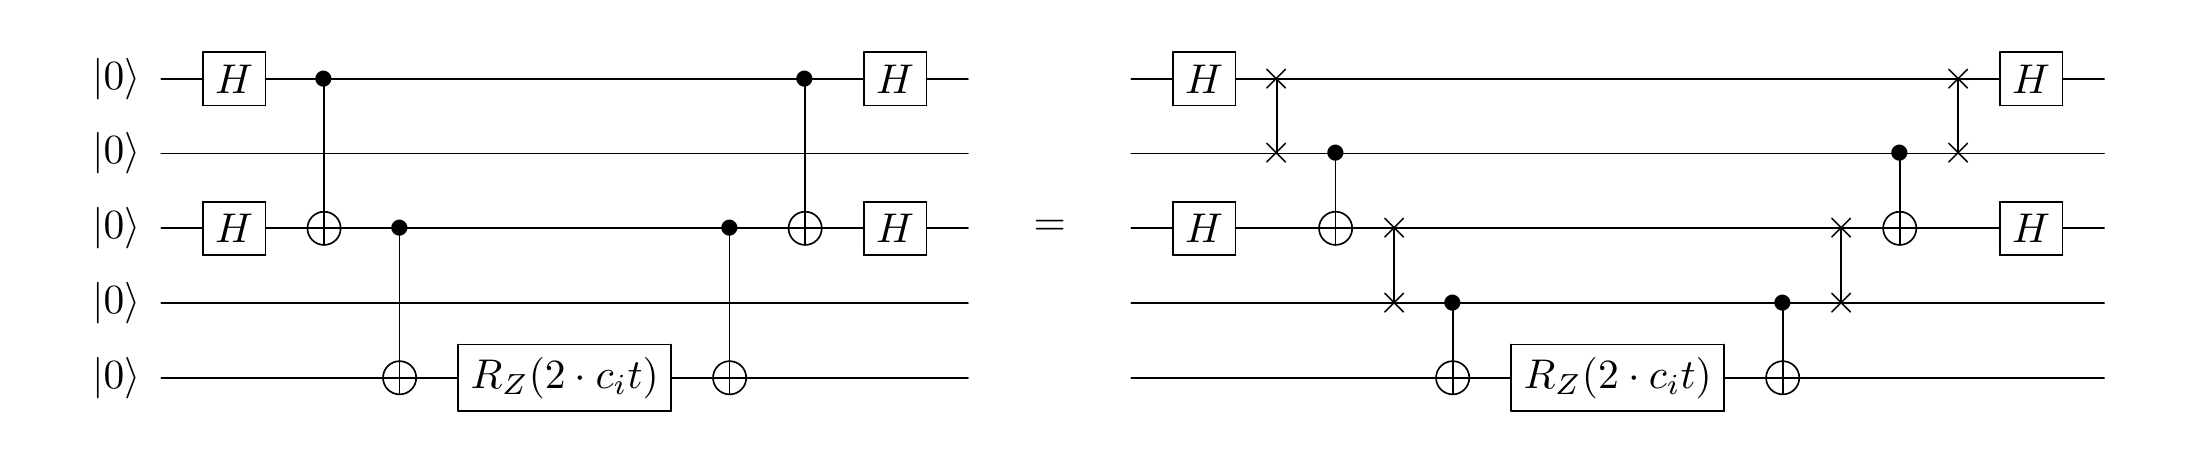}}
        \end{minipage}
    \caption{\textit{Example of Pauli strings with identity matrices exponentiation on a quantum circuit. Terms respectively from the top are $XIZ$, $XIIZ$, $XIXIX$.}}
    \label{fig:Pauli term exp. on circuit with ID terms example}
\end{figure}

That means, that the final circuit depth depends on the structure of the Pauli term, not only its weight. In the worst-case scenario, the 2-qubit gate complexity is $O(n)=6(n-1)+2$ where n is a number of qubits. Further optimizations are possible. To name a few: the simplest would be cancellation of the gates from the adjacent terms sections in the circuit. If the single-term section ends with e.g. a Hadamard or CNOT gate and the other section begins with them on the same qubits, those gates can be canceled out. This technique is usually automatically applied within transpilers. A more advanced method is simultaneous diagonalization\cite{Berg2020}, i.e., application group of the commuting terms using fewer gates than it would be with the sequential exponentiation of the terms. For this method to be visibly effective, the commuting terms need to be grouped together, changing radically the order of the original terms sequence, which may strongly influence the final state for the small number of Trotter steps. In the end, promising results in circuit reduction were also shown in this work \cite{Mukhopadhyay2023}.

\newpage
\section{Qubit mapping comparison}
\label{SI_sec:qubit_mapping_comparison}

During testing methods reducing circuits, the generic qubit mapping methods were checked: Jordan-Wigner (JW), Bravyi-Kitaev (BK), and Parity mappings. By comparing circuits in Figure \ref{fig: qubit mappings comparison}, for full Hamiltonian from generic Trotterization with 1 Trotter steps, there are no significant differences between those 3 for $<$30 qubits, from where BK started to produce shallower circuits. It agrees with a broader study on the quantum chemistry dataset comparing JW to BK \cite{Tranter2018}.

\begin{figure}[h!]
\centering
\includegraphics[width=\linewidth]{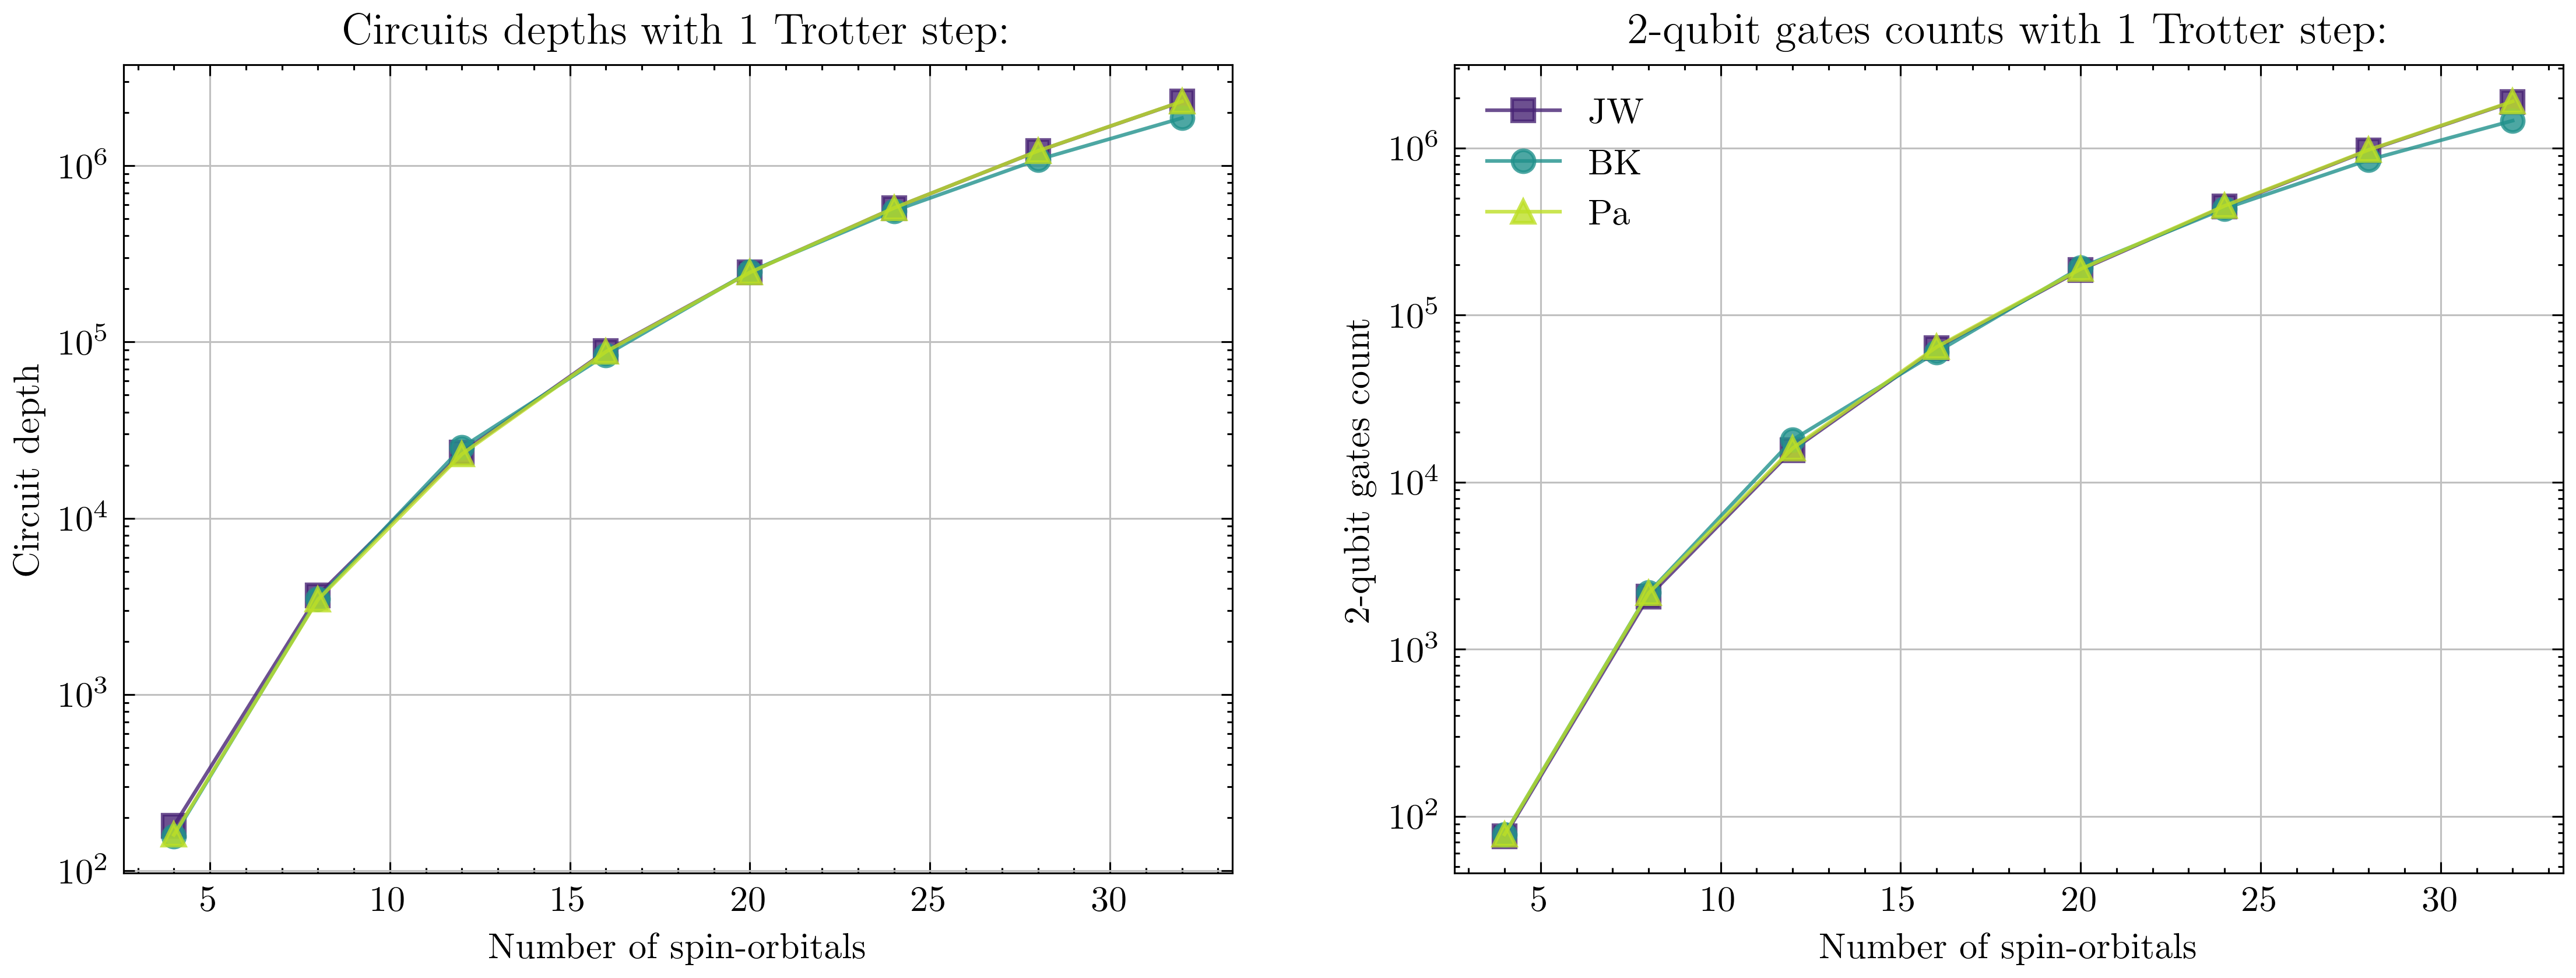}
\caption{\textit{Circuit depth and number of 2-qubit gates comparison on circuits yielded by first-order 1 Trotter step PF with $Clifford+R_z$ gates only for Jordan-Wigner (JW), Bravyi-Kitaev (BK) and Parity (Pa) mappings.
}}
\label{fig: qubit mappings comparison}
\end{figure}

Since the focus in this work is on low number-of-qubits regimes, the JW mapping was chosen. All previous results in the main part of the paper were produced with it. Additionally, to check potential differences between the mappings for methods reducing circuits from Trotterization, all results were generated for BK and Parity mappings as well and shown in Section~SI~\ref{SI_sec:detailed circuti reduction results}.

\newpage
\section{Circuit depth reduction methods}
\label{SI_sec:circuit_depth_reduction_methods}

\subsection{Hamiltonian terms truncation}
\label{SI_subsec:hamiltonian_terms_truncation}

The number of terms in the qubit mapped Hamiltonian linearly contributes to the circuit depth in the first-order PF, which makes it challenging to both simulate and run on the real devices with each increase in the active space size of the simulated system. For the targeted covalent drugs use case, similarly to most of the use cases leveraging time evolution dynamics of the quantum chemistry systems, only the arbitrary initial time range of the observable trajectory is taken into consideration. That means that Hamiltonian terms with small coefficients will not noticeably influence the final observable within the chosen time range and can be neglected. Let us show it on single term single-qubit Hamiltonian $\hat{H}_p=c _H\hat{P}_H$ example and single term, single-qubit observable $\hat{A}=\hat{P}_A$ . For simplicity reasons, let us consider $\hat{P}_H=\hat{\sigma}_x$ and $\hat{P}_A=\hat{\sigma}_z$.

For the state $\left|\psi\right\rangle$ and observable $\hat{A}$, the expectation value of the $\hat{A}$ is defined as:
$$
\langle\hat{A}\rangle=\langle\psi|\hat{A}|\psi\rangle
$$
The measured state is time-evolved state from arbitrarily chosen initial state $\left|\psi_{init}\right\rangle$:
$$
\left|\psi\right\rangle=\ e^{i{\hat{H}}_pt}\left|\psi_{init}\right\rangle=e^{i\left(c_1{\hat{\sigma}}_x\right)t}\left|\psi_{init}\right\rangle
$$
$$
e^{i\left(c_1{\hat{\sigma}}_x\ \right)t}=\sum_{j=0}^{\infty}\frac{\left(-ic_1t\right)^j}{j!}\ {\hat{\sigma}}_x^j=\sum_{j=0}^{\infty}\frac{\left(-1\right)^j\left(c_1t\right)^{2j}}{(2j)!}\ \hat{I}+\sum_{j=0}^{\infty}\frac{{-\left(-1\right)}^j\left(c_1t\right)^{2j+1}}{(2j+1)!}\ {\hat{\sigma}}_x=\cos{\left(c_1t\right)}\hat{I}-i\sin{\left(c_1t\right)}{\hat{\sigma}}_x\ 
$$
And with the representation in the computational basis:
$$
\left|\psi_{init}\right\rangle= \left[\begin{matrix} \alpha_0 \\ \alpha_1 \\\end{matrix}\right]
$$
$$
e^{i(c_1{\hat{\sigma}}_x)t}=\cos{(c_1t)}\hat{I}-i\sin{(c_1t)}{\hat{\sigma}}_x=\left[\begin{matrix}\cos{\left(c_1t\right)}&-i\sin{\left(c_1t\right)}\\-i\sin{\left(c_1t\right)}&\cos{\left(c_1t\right)}\\\end{matrix}\right],
$$
what is exactly $R_x(2\cdot c_1t)$, which is applied in the circuit.
$$
|\psi\rangle=\left[\begin{matrix} \cos{(c_1t)}& -i\sin{(c_1t)} \\ -i\sin{(c_1t)}& \cos{(c_1t)} \\\end{matrix}\right] 
\left[\begin{matrix} \alpha_0 \\ \alpha_1 \\\end{matrix}\right] =
 \left[\begin{matrix} cos(c_1 t) \alpha_0 -i sin(c_1 t) \alpha_1 \\ -i sin(c_1 t) \alpha_0 + cos(c_1 t) \alpha_1 \\\end{matrix}\right]
$$
That gives the formula for the expectation value:
$$
\langle\hat{A}\rangle=\langle\psi|{\hat{\sigma}}_z|\psi\rangle
$$
$$
\langle\hat{A}\rangle = \left[\begin{matrix}{\cos(c_1t)\alpha}_0^\ast+i\sin(c_1t)\alpha_1^\ast & i\sin{(c_1t)\alpha_0^\ast+{\cos{(c_1t)}\alpha}_1^\ast}\\\end{matrix}\right] \left[\begin{matrix} 1 & 0 \\ 0 & -1 \\\end{matrix}\right]
 \left[\begin{matrix} cos(c_1 t) \alpha_0 -i sin(c_1 t) \alpha_1 \\ -i sin(c_1 t) \alpha_0 + cos(c_1 t) \alpha_1 \\\end{matrix}\right]
$$
$$
\langle\hat{A}\rangle=\cos(2c_1t)(|\alpha_0|^2-|\alpha_1|^2)+i sin(2c_1 t) (\alpha_0 \alpha_1^*-\alpha_0^* \alpha_1)
$$
that means the period of the observable’s expectation value is $\pi/c_1$, so the higher the terms’ coefficient, the higher the frequency of a an observable potential variation induced by the term. Now, to assess if the term in Hamiltonian can be skipped, the maximum change induced by the term to the observable needs to be accessed:
$$
\frac{d\langle\hat{A}\rangle}{dt}=-2c_1(\sin(2c_1t)(|\alpha_0|^2-|\alpha_1|^2)-i cos(2 c_1 t) (\alpha_0 \alpha_1^*-\alpha_0^* \alpha_1))
$$
Since $|\alpha_0|^2+|\alpha_1|^2$ needs to be 1, there expression simplify to:
$$
\frac{d\langle\hat{A}\rangle}{dt}=-2c_1(\sin{({2c}_1t})(1-2\left|\alpha_1|^2\right)-i\ cos\left(2c_1t\right)\left(\alpha_0\alpha_1^\ast-\alpha_0^\ast\alpha_1\right))
$$
Then, to calculate the maximum value with respect to the initial state, the global phase can be neglected and the $\alpha_0$ may be chosen as the real amplitude. That means that the second term will yield the maximum absolute value if the $\alpha_1$ is imaginary. This condition is fulfilled by the initial states across the Z-Y axes plane of the Bloch sphere – perpendicular to the X axis. Those two specifications allow to yield the formula dependent only on the single amplitude:
$$
\max_{(\alpha_0,\alpha_1)}{\left(\left|\frac{d\langle\hat{A}\rangle}{dt}\right|\right)}=
\max_{\alpha_1}\left(\left|2c_1\left(\sin{({2c}_1t}\right)\ (1-2\left|\alpha_1|^2\right)\pm2\ cos\left(2c_1t\right)\sqrt{1-Im\left(\alpha_1\right)^2}\ Im\left(\alpha_1\right)\ )\right|\right)
$$
First term gives the largest value $2c_1$ (for $t=\frac{\pi}{4c_i}(1+2n)$) for the ${|\alpha}_1|^2\in{0,\ 1}$, the second gives the same largest value (for $t=\frac{n\pi}{2c_i}$) for $\alpha_1\in\{\frac{i}{\sqrt2},\ \frac{-i}{\sqrt2}\}$. The numerical evaluation also yielded the largest value $2c_1$ for the possible space of $\alpha_1$ and $t$:

\begin{figure}[h!]
\centering
\includegraphics[width=0.8\linewidth]{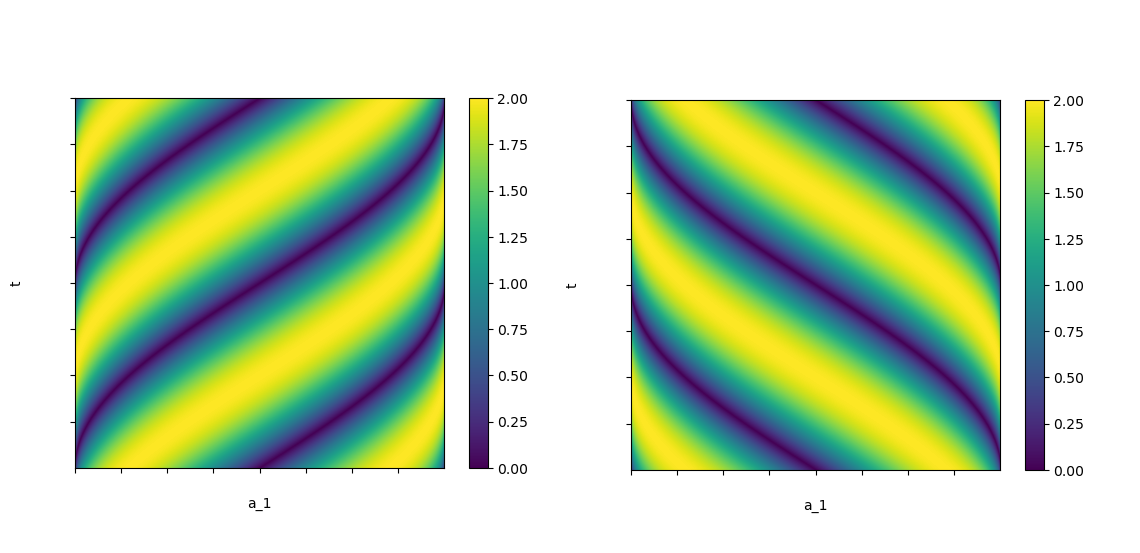}
\caption{\textit{$\frac{d\langle\hat{A}\rangle}{dt}$ numerical evaluation from $t$ and $\alpha_1$ amplitude.}}
\label{fig:numerical evaluation of obs. from state change}
\end{figure}

In this way, the worst-case scenario of the observable expectation variation $d\langle\hat{A}\rangle$ of the Hamiltonian’s term with coefficient $c_1$ for a given time range $dt$ is:
$$
\max{(d\langle\hat{A}\rangle)}= 2c_1 dt
$$
Let us generalize this example to Hamiltonian with any number of terms acting on many qubits. Based on this formula, the truncation algorithm may be set, cutting off the given Hamiltonian’s terms. The threshold will be set for the coefficients $c_0$, below which the terms will be neglected as they should not influence any observable expectation value more than given acceptable value $\epsilon_{d\langle\hat{A}\rangle}$ :
$$
c_0=\frac{\epsilon_{d\langle\hat{A}\rangle}}{2dt}
$$

For example, for the $\epsilon_{d\langle\hat{A}\rangle}=1\%$ and time range of 0-10 time (a.u.), the acceptable threshold is $c_0=0.0005$. A schematic representation of the truncation algorithm through pseudocode is shown in Figure \ref{alg:truncation alg. description} below.

\FloatBarrier
\begin{figure}[h]
    \includegraphics{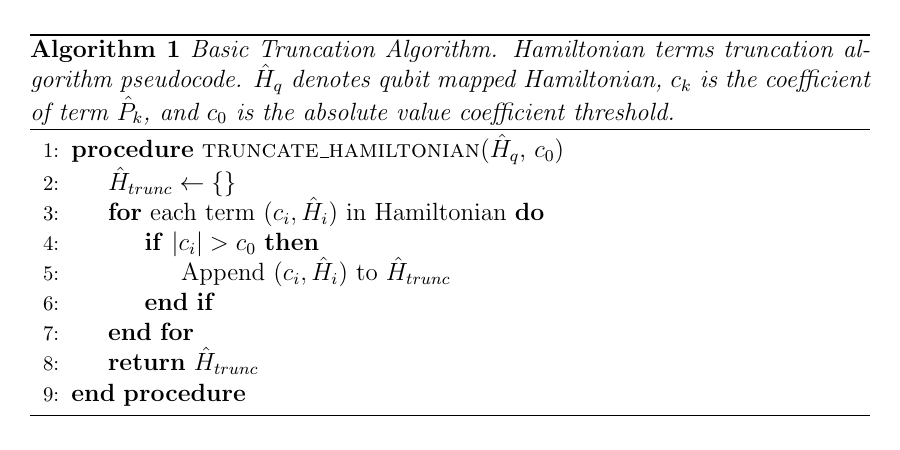}
    \caption{\textit{Pseudocode for a basic implementation of Hamiltonian terms truncation algorithm.}}
    \label{alg:truncation alg. description}
\end{figure}

\FloatBarrier
\newpage

\subsection{Qubit tapering}
\label{SI_subsec:qubit_tapering}

Qubit tapering is the technique leveraging the ${Z}_2$ symmetries in molecular Hamiltonians to perform the Hamiltonian simulation using fewer qubits and, in some cases, with shallower circuits. Fundamentally, the original qubit Hamiltonian ${\hat{H}}_q$ is transformed as:
$$
{\hat{H}}_q=\ \sum_{k=1}^{K}{c_k{\hat{P}}_k}
$$
into new Hamiltonian ${\hat{H}}^\prime_q$, which will have the same eigenvalues as ${\hat{H}}_q$, using unitary operator\ $\hat{U}$:
$$
\hat{H}^\prime_q=\ {\hat{U}}^\dagger{\hat{H}}_q\hat{U}=\ \sum_{k=1}^{K}{c^\prime_k \hat{P}^\prime_k}
$$
but with each of the terms $\hat{P}^\prime_k$ containing the same Paulis acting on a subset of qubits. To illustrate it, let us take:
$$
\hat{H}^\prime ={\hat{\sigma}}_x\otimes{\hat{\sigma}}_z-\ \hat{I}\otimes{\hat{\sigma}}_z
$$
All the terms apply on the second qubit the ${\hat{\sigma}}_z$ operator. In that case, the Hamiltonian can be rewritten as:
$$
\hat{H}^\prime =\left({\hat{\sigma}}_x\otimes\hat{I}-\ \hat{I}\otimes\hat{I}\right)\hat{I}\otimes{\hat{\sigma}}_z
$$
yielding two tapered Hamiltonians with the eigenvalues of ${\hat{\sigma}}_z$ as the\ prefactor:
$$
{\hat{H}}_{tapered}\ =\pm1({\hat{\sigma}}_x-\hat{I})
$$
with the Paulis acting on the first qubit only. This way, for two eigenvalues from each of the 1-qubit ${\hat{H}}_{tapered}$, there are in total 4 eigenvalues being the eigenvalues of the 2-qubit $\hat{H}^\prime_q$. 2 qubits are ‘tapered’ out and the cost of the Hamiltonian exponentiation on the circuit for the potential simulation is reduced. The challenge lies in finding the original Hamiltonian ${\hat{H}}_q$ symmetries, and then the preparation of $\hat{H}^\prime_q$ from ${\hat{H}}_q$ by leveraging found symmetries to taper as much qubits as possible. Methods for this were described first in \cite{Bravyi2017}, with the extension in \cite{Setia2020}. For the results in this paper, the Qiskit’s \href{https://docs.quantum.ibm.com/api/qiskit/qiskit.quantum_info.Z2Symmetries}{Z2Symmetries} class was used with the original tapering method implementation\cite{Bravyi2017}. 
\newpage

\subsection{Clifford Decomposition and Transformation (CDAT)}
\label{SI_subsec:CDAT}

Clifford Decomposition and Transformation (CDAT) is the procedure described in \cite{Gujarati2023}. During the simulating circuit creation, given steps are taken iteratively: taking the Pauli term $c_k{\hat{P}}_k$ from qubit mapped Hamiltonian with evolution time t, exponentiate them on the circuit ${\hat{V}}_k\left(\theta_k\right)=e^{-i\theta_k{\hat{P}}_k\ }$, where $\theta_k=c_kt$, and then using a few quantum gates identities\cite{Gujarati2023} the circuit is transformed in such a way, that it can be decomposed into Clifford part ${\hat{C}}_k$ (containing only Clifford gates, hence non-parametrized) and non-Clifford part ${\hat{U}}_k\left(\theta_k\right)$ (containing Clifford and non-Clifford gates) giving ${\hat{V}}_k\left(\theta_k\right)={\hat{C}}_k{\hat{U}}_k(\theta_k)$, so the non-Clifford part is applied in the decomposed circuit first. Then the Clifford gates ${\hat{C}}_k$ are taken from the decomposed circuit and used to transform the remaining Paulis and all the measurement operators. Since, the ${\hat{C}}_k$ is already applied, the non-Clifford part ${\hat{U}}_k(\theta_k)$ can be applied to the already existing circuit from previous terms, and the process is repeated for the rest of the Paulis in the Hamiltonian. Single term transformation example is shown in the Figure \ref{fig:CDAT alg. example}.

\begin{figure}[h!]
    \centering
    \includegraphics[width=1\linewidth]{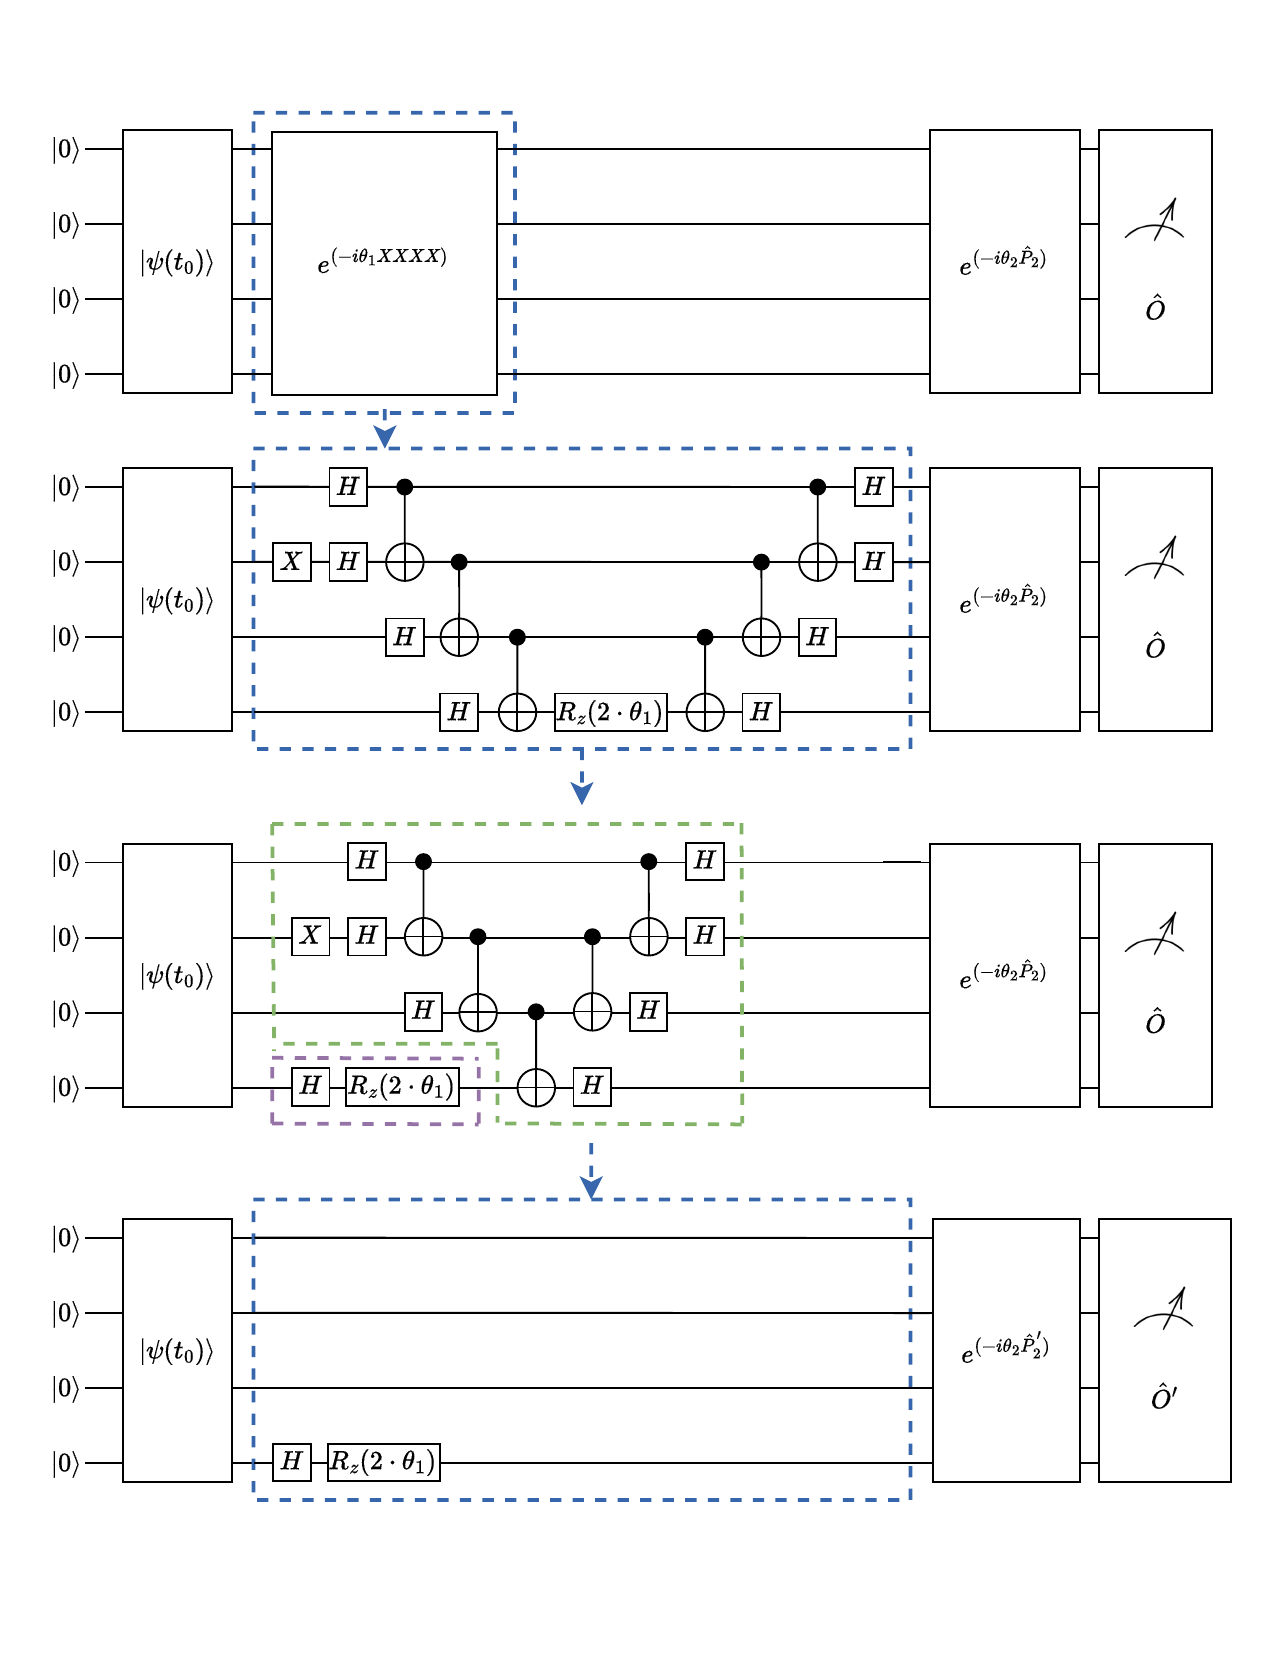}
    \caption{\textit{Example of single CDAT step on 4 qubits time-evolution circuit.}}
    \label{fig:CDAT alg. example}
\end{figure}
\FloatBarrier

\newpage
\section{Detailed circuit reduction results}
\label{SI_sec:detailed circuti reduction results}

\subsection{Clifford Decomposition and Transformation (CDAT)}
\label{SI_subsec:CDAT with qubit mapping}

CDAT gives similar, systematic reduction both for circuit depth and 2-qubit gates.

\begin{figure}[h!]
\centering
\includegraphics[width=0.98\linewidth]{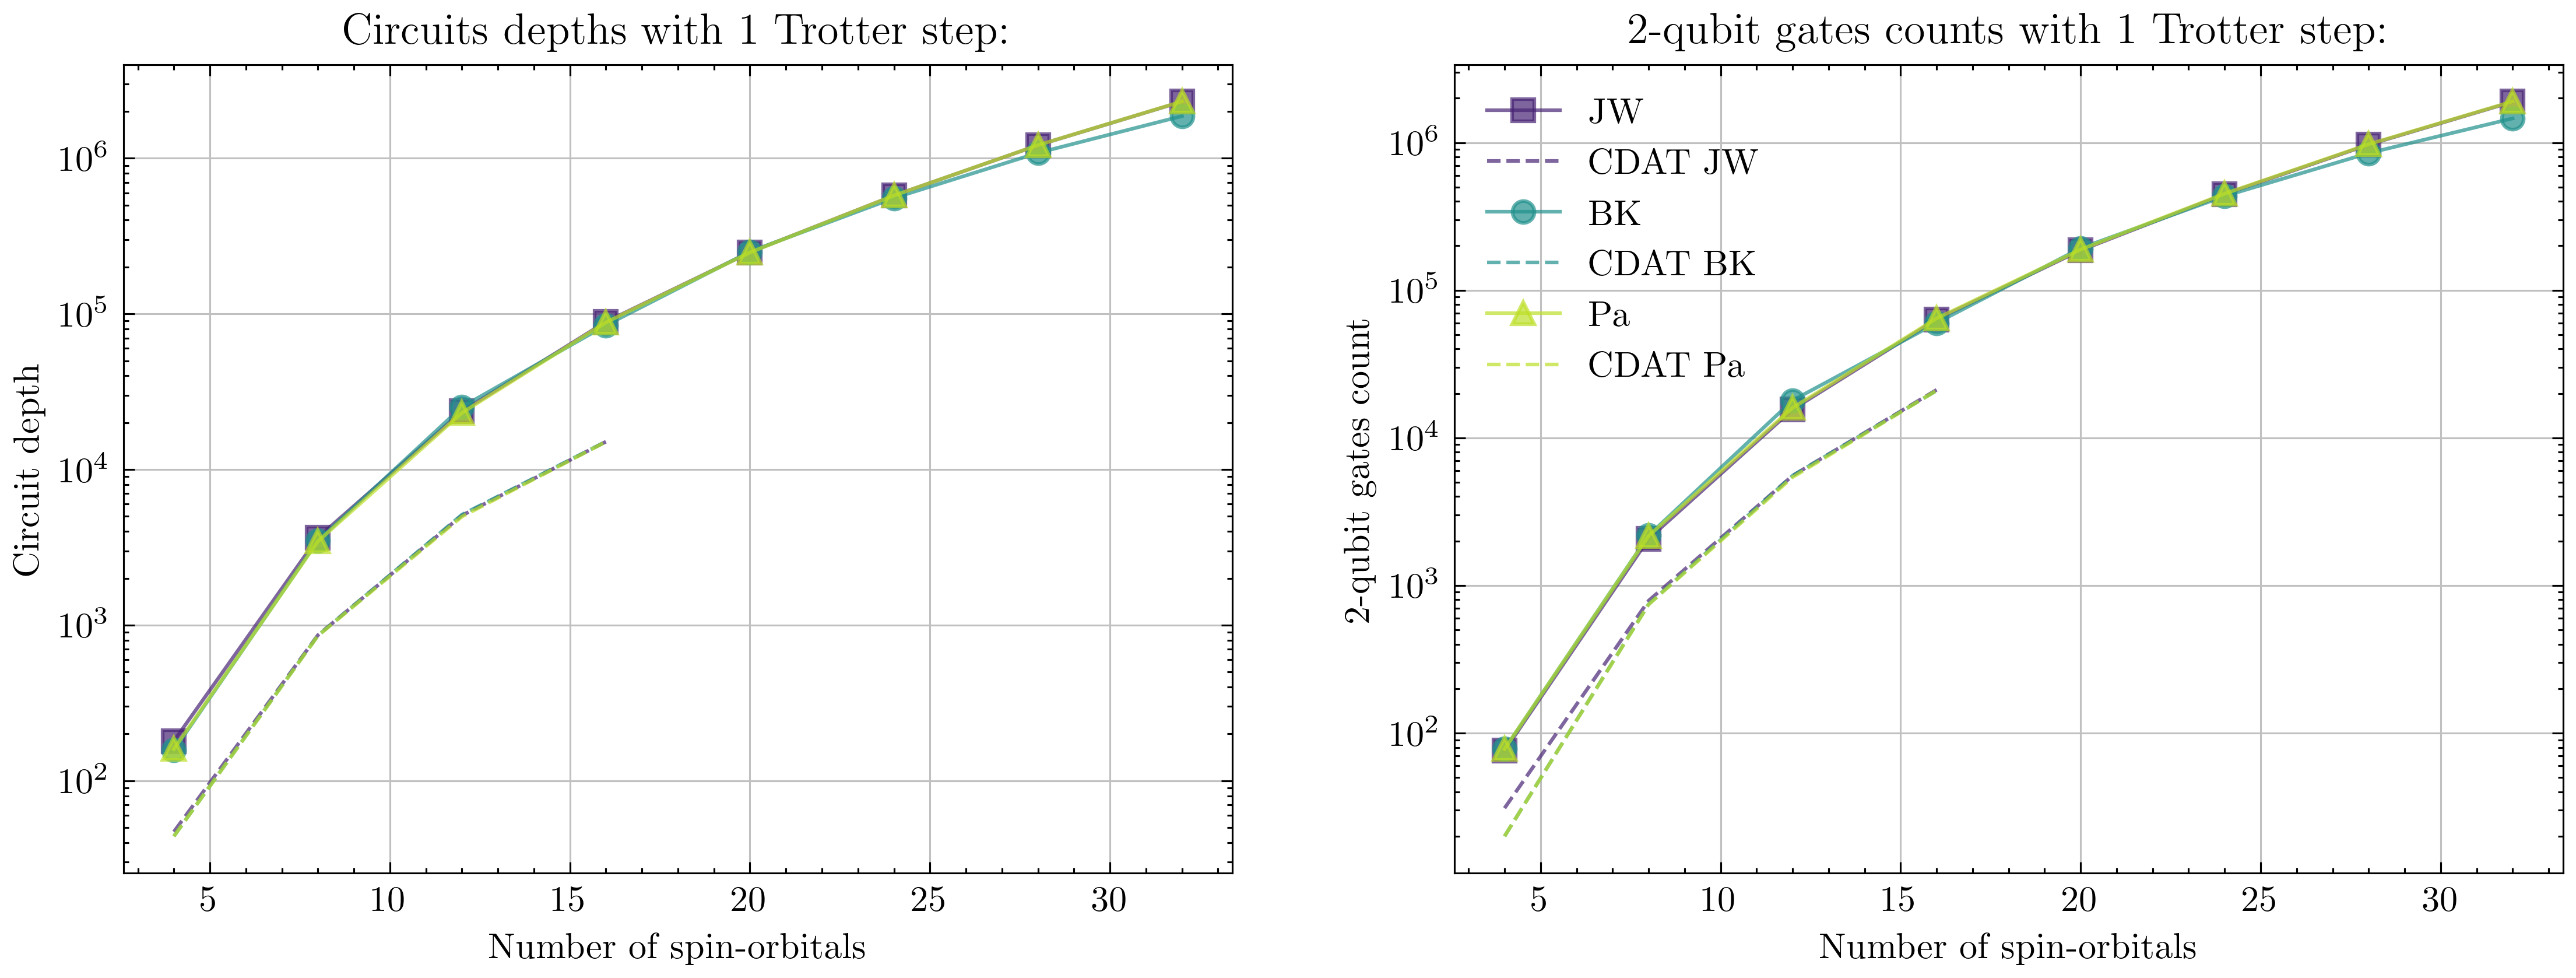}
\caption{\textit{Circuit depths and number of 2-qubit gates comparison with and without CDAT applied for different qubit mappings.}}
\label{fig:CDAT circuit reduction results}
\end{figure}
\FloatBarrier
\newpage

\subsection{Qubit Tapering}
\label{SI_subsec:Tapering with qubit mapping}

All results for qubit tapering are taken as a mean from all subexperiments. In all cases, the number of terms stayed on a similar level both in the Hamiltonian and the measurement operator. The circuit depth results vary in the small active space sizes for different qubit mappings. Besides that, the depths from different mappings are close to each other. 

\begin{figure}[h!]
\centering
\includegraphics[width=0.98\linewidth]{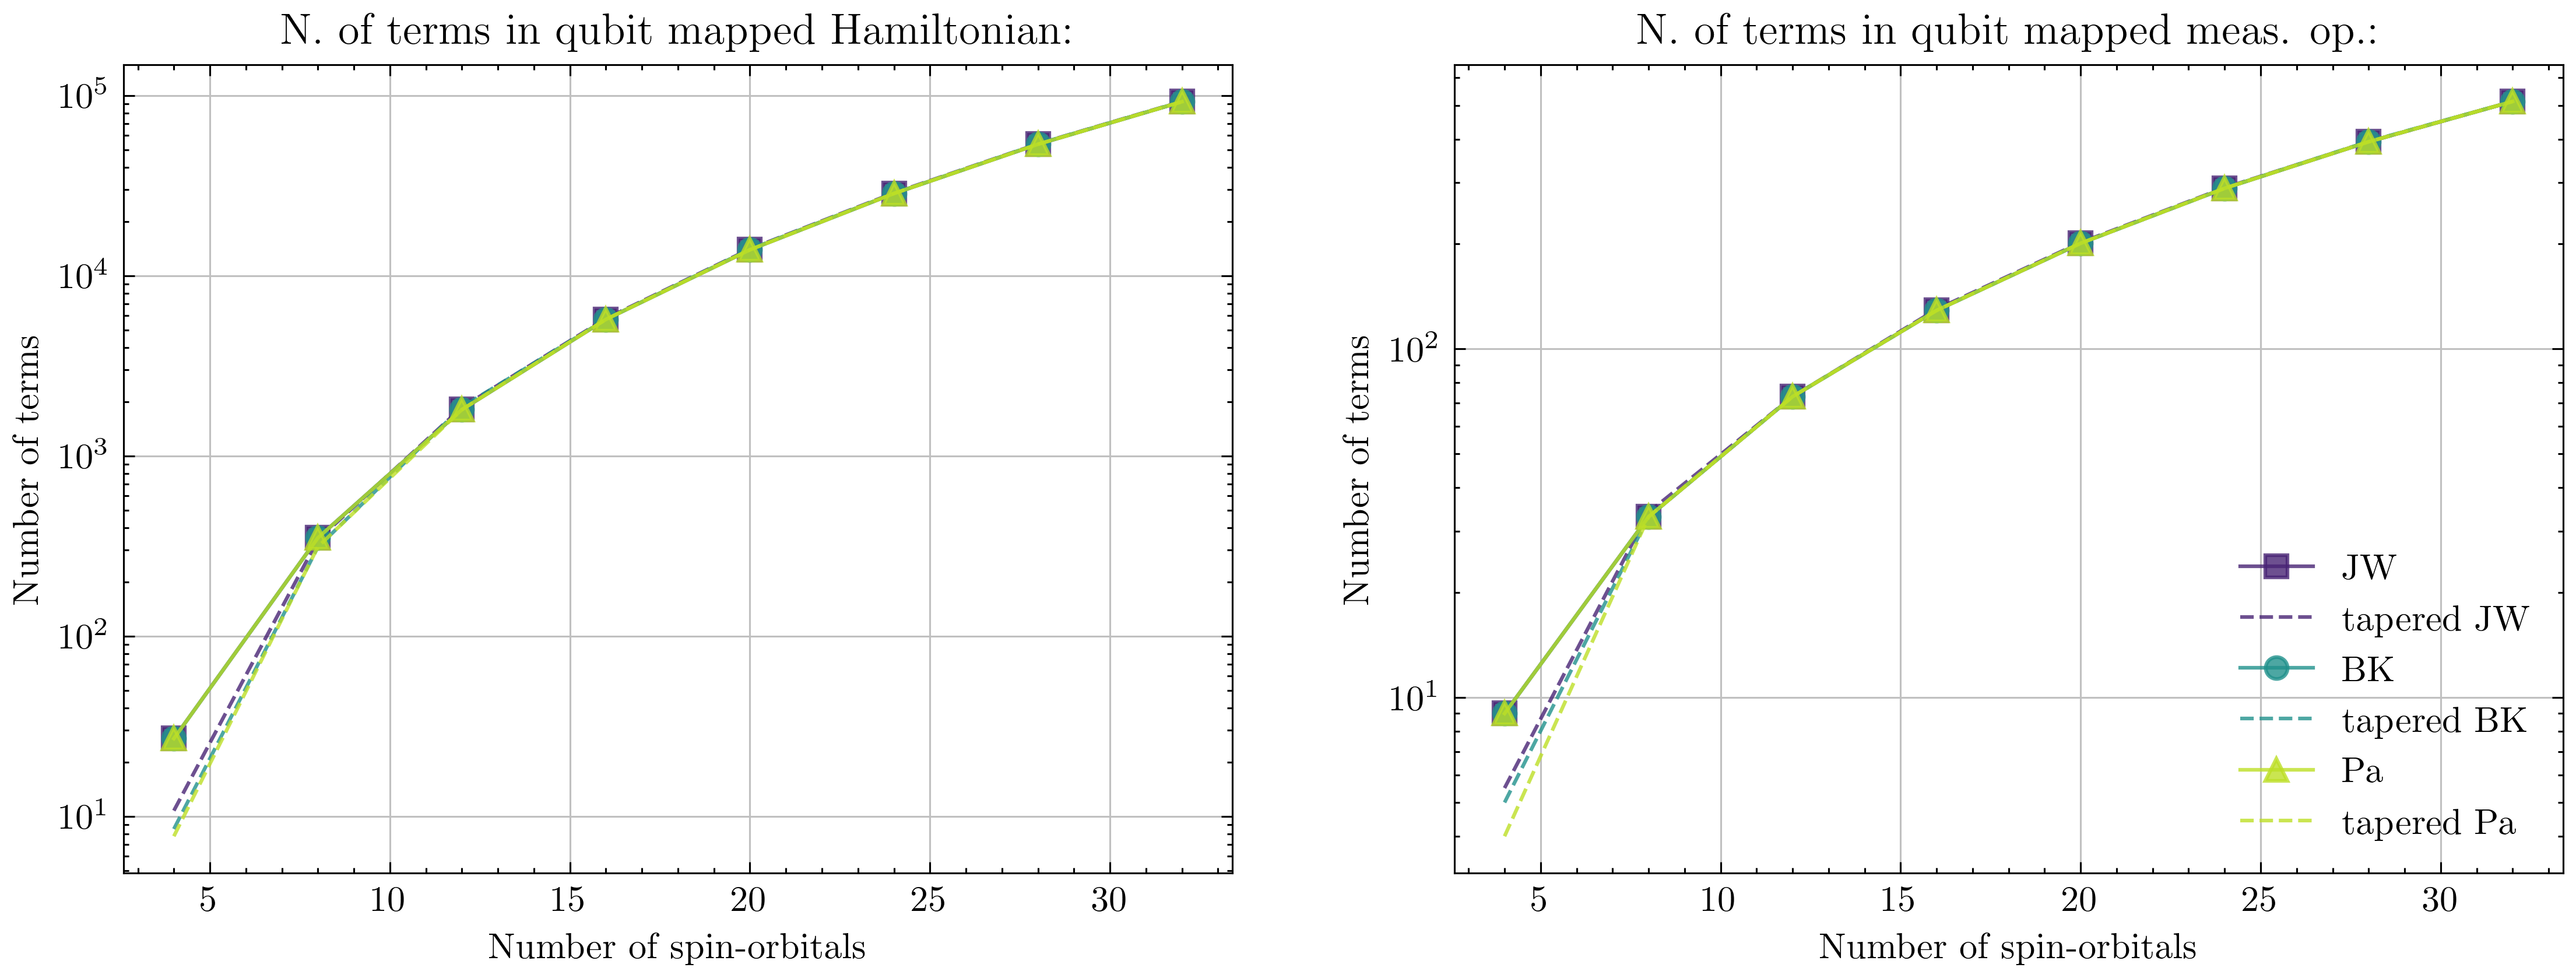}
\caption{\textit{Number of terms in Hamiltonian and measurement observable comparison with and without qubit tapering applied for different qubit mappings.}}
\label{fig:Tapering operators reduction results}
\end{figure}

\begin{figure}[h!]
\centering
\includegraphics[width=0.98\linewidth]{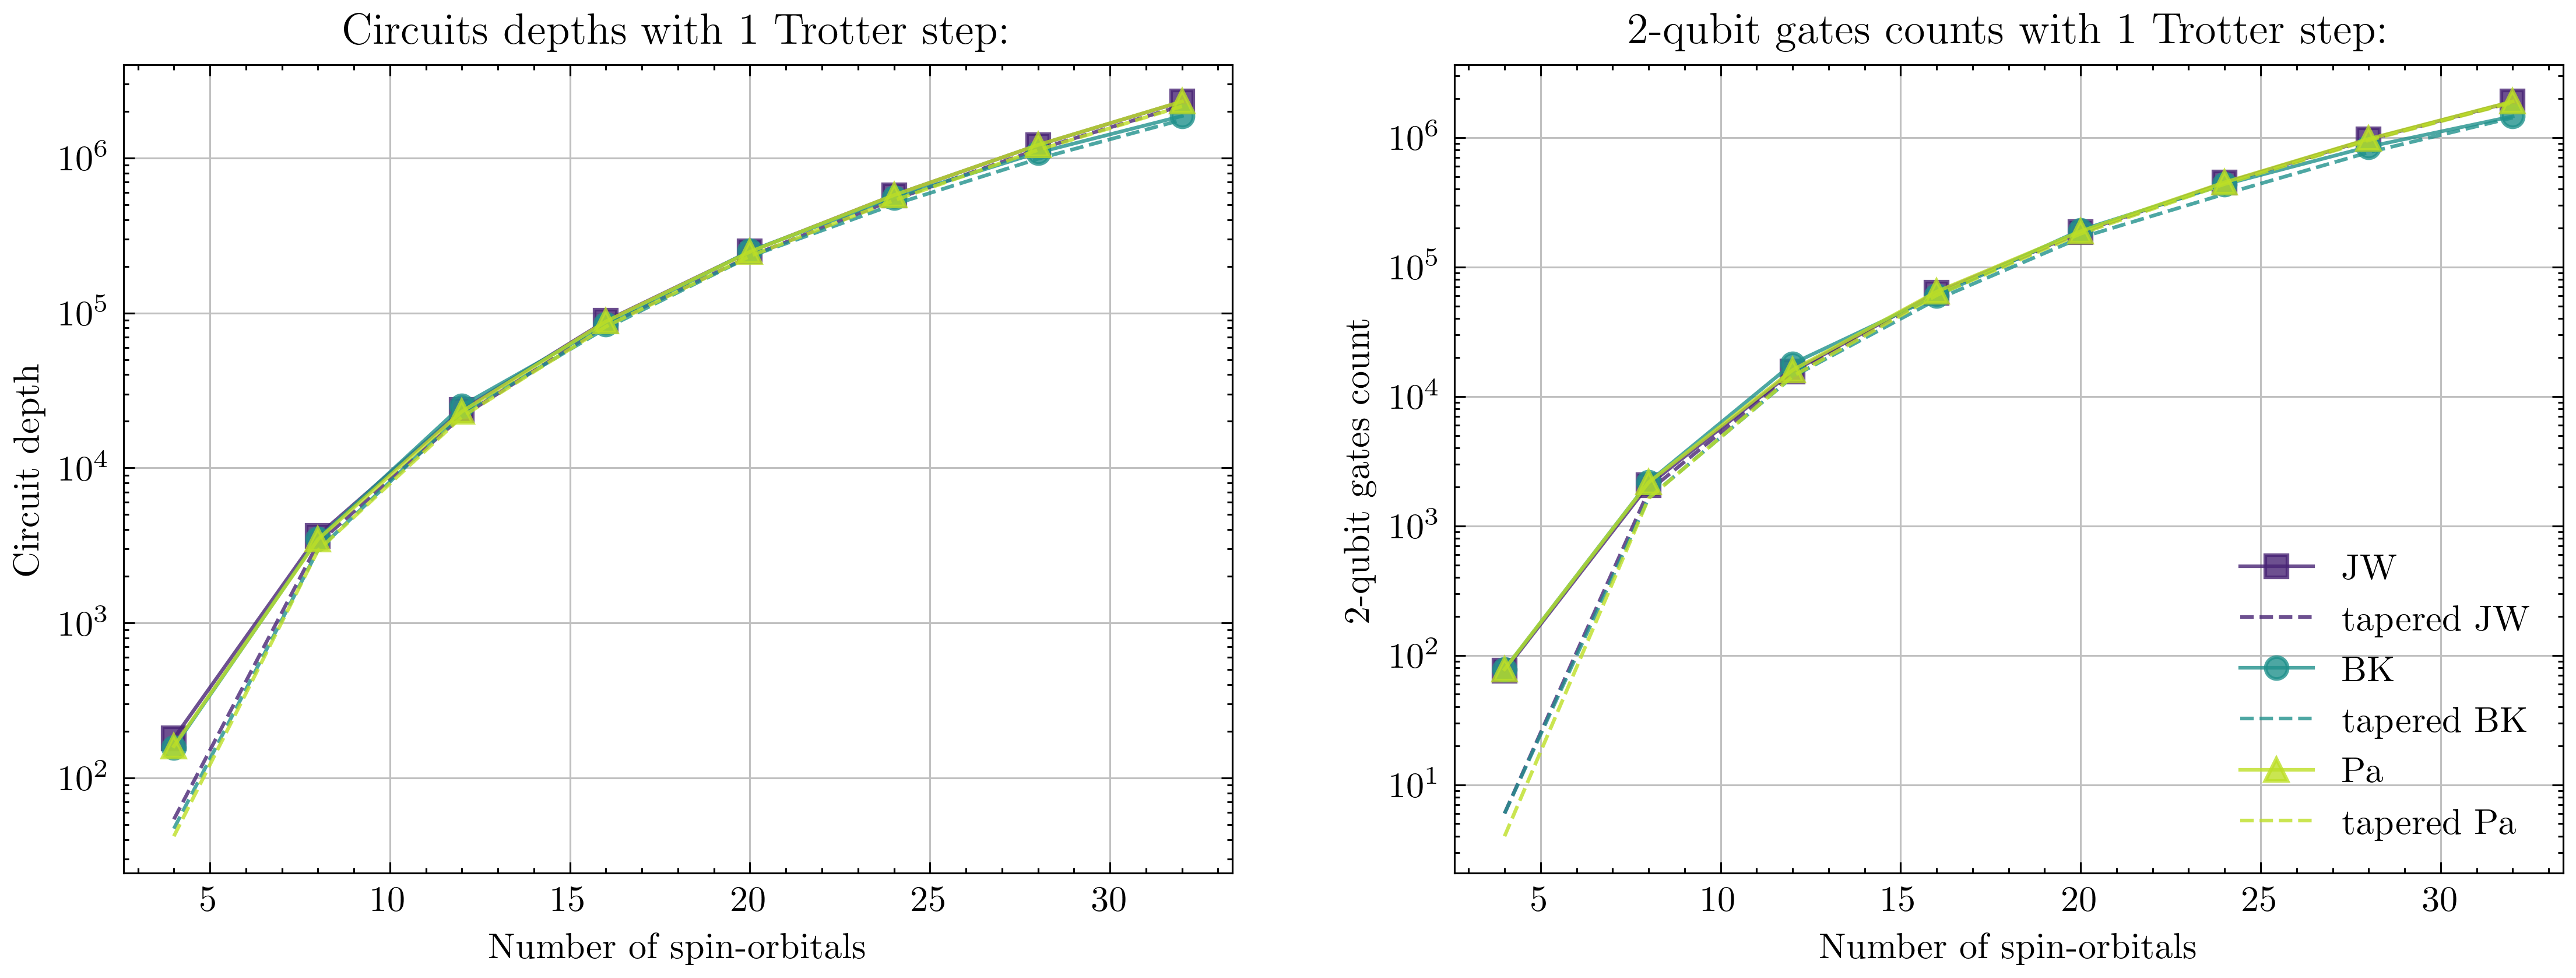}
\caption{\textit{Circuit depths and number of 2-qubit gates comparison with and without qubit tapering applied for different qubit mappings.}}
\label{fig:Tapering circuit reduction results}
\end{figure}
\FloatBarrier
\newpage

\subsection{Comparison of the combinations}
\label{SI_subsec:Tapering and CDAT with qubit mapping}

Additionally, the combination of the tapering and CDAT (tapering applied first) was checked for potential improvements. The two plots below show the comparison to CDAT or qubit tapering applied only. A combination of this too yields significantly smaller circuits, than just the tapering, but in comparison to CDAT only, it is a little bit worse for 8+ qubits.

\begin{figure}[h!]
\centering
\includegraphics[width=0.98\linewidth]{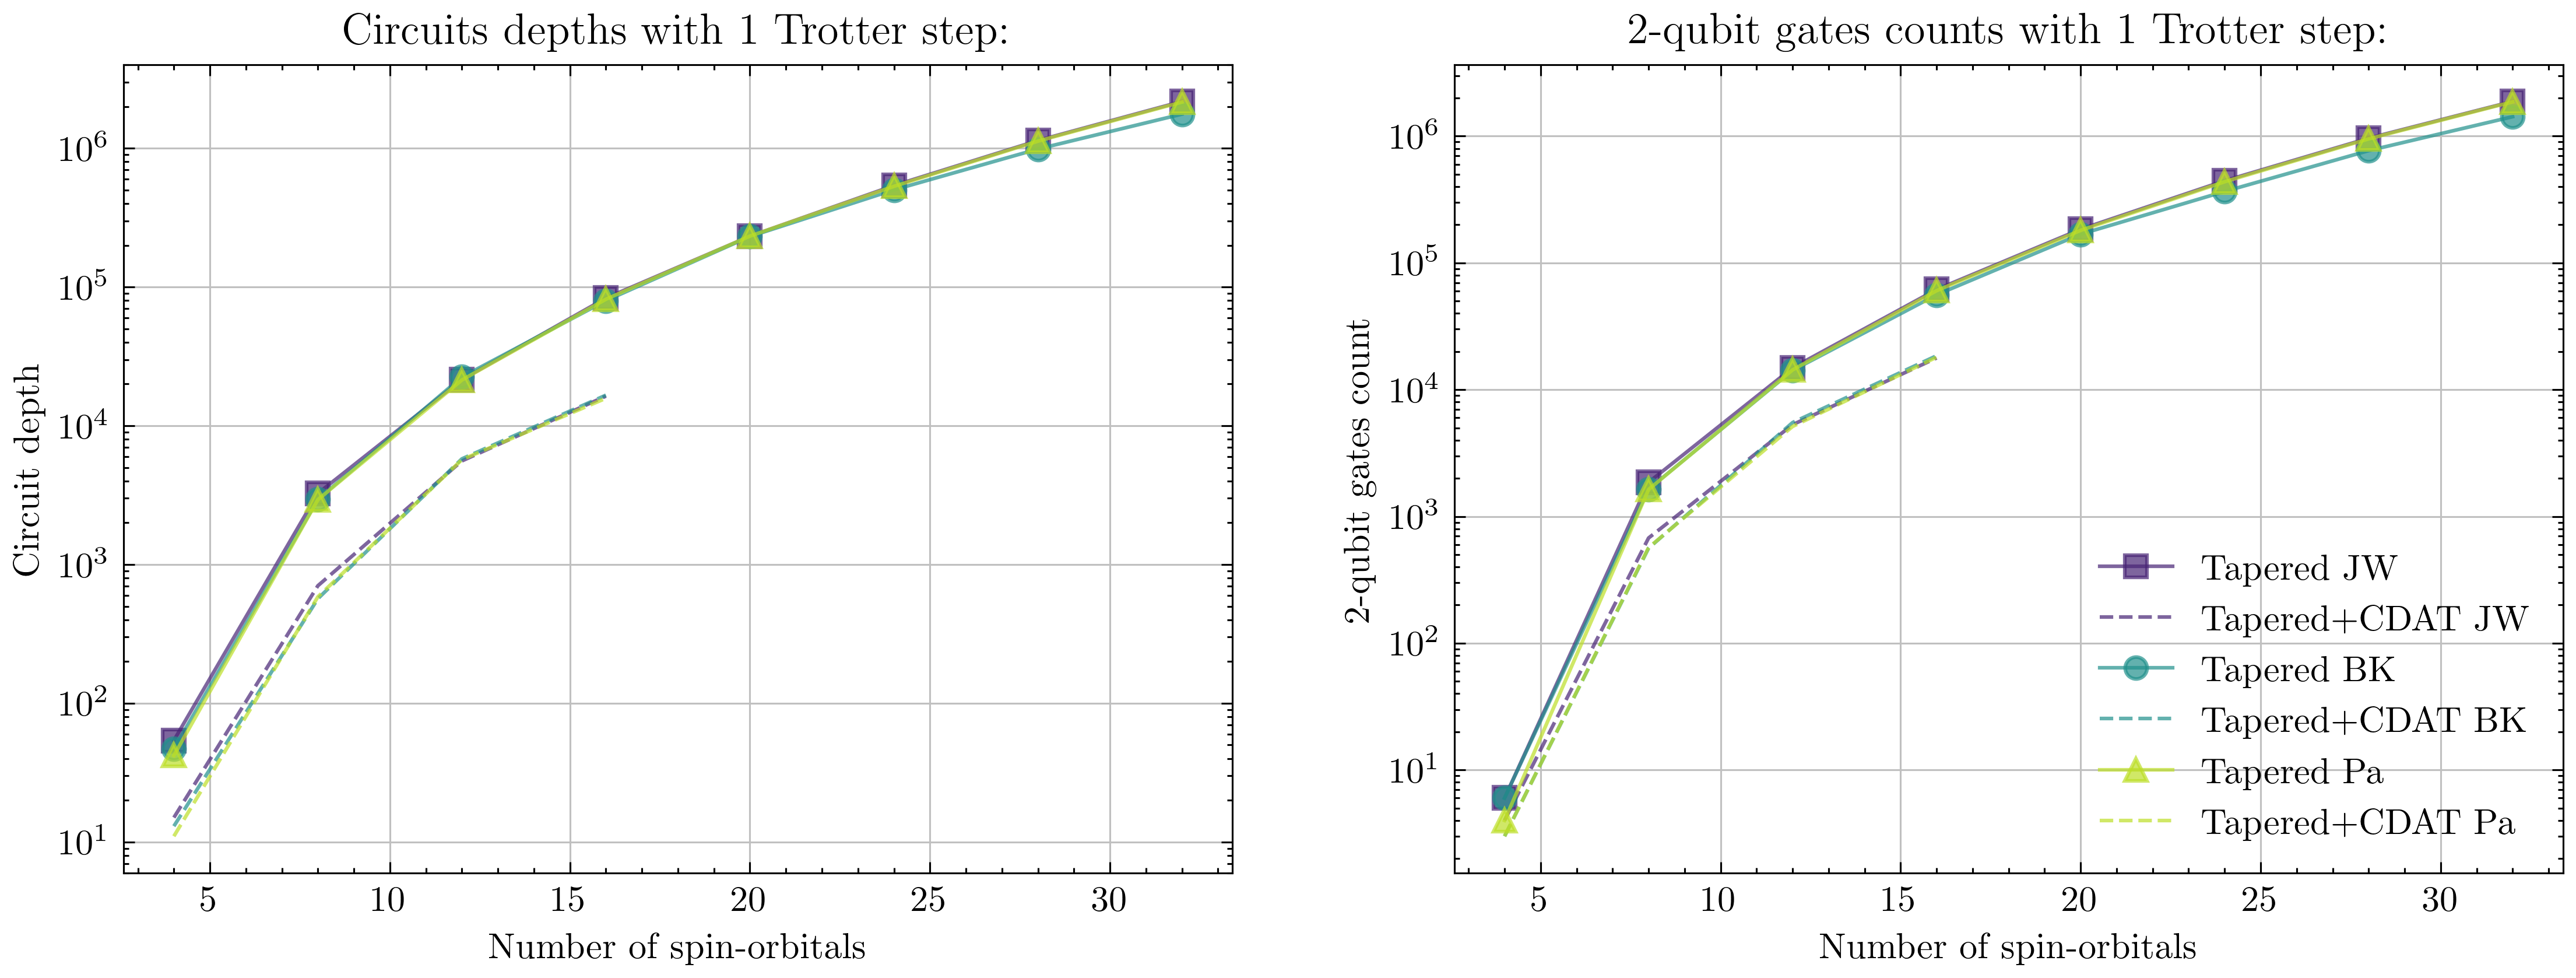}
\caption{\textit{Circuit depths and a number of 2-qubit gates comparison with qubit tapering applied only and with qubit tapering and CDAT applied for different qubit mappings.}}
\label{fig:Tapering+CDAT circuit reduction results}
\end{figure}

\begin{figure}[h!]
\centering
\includegraphics[width=0.98\linewidth]{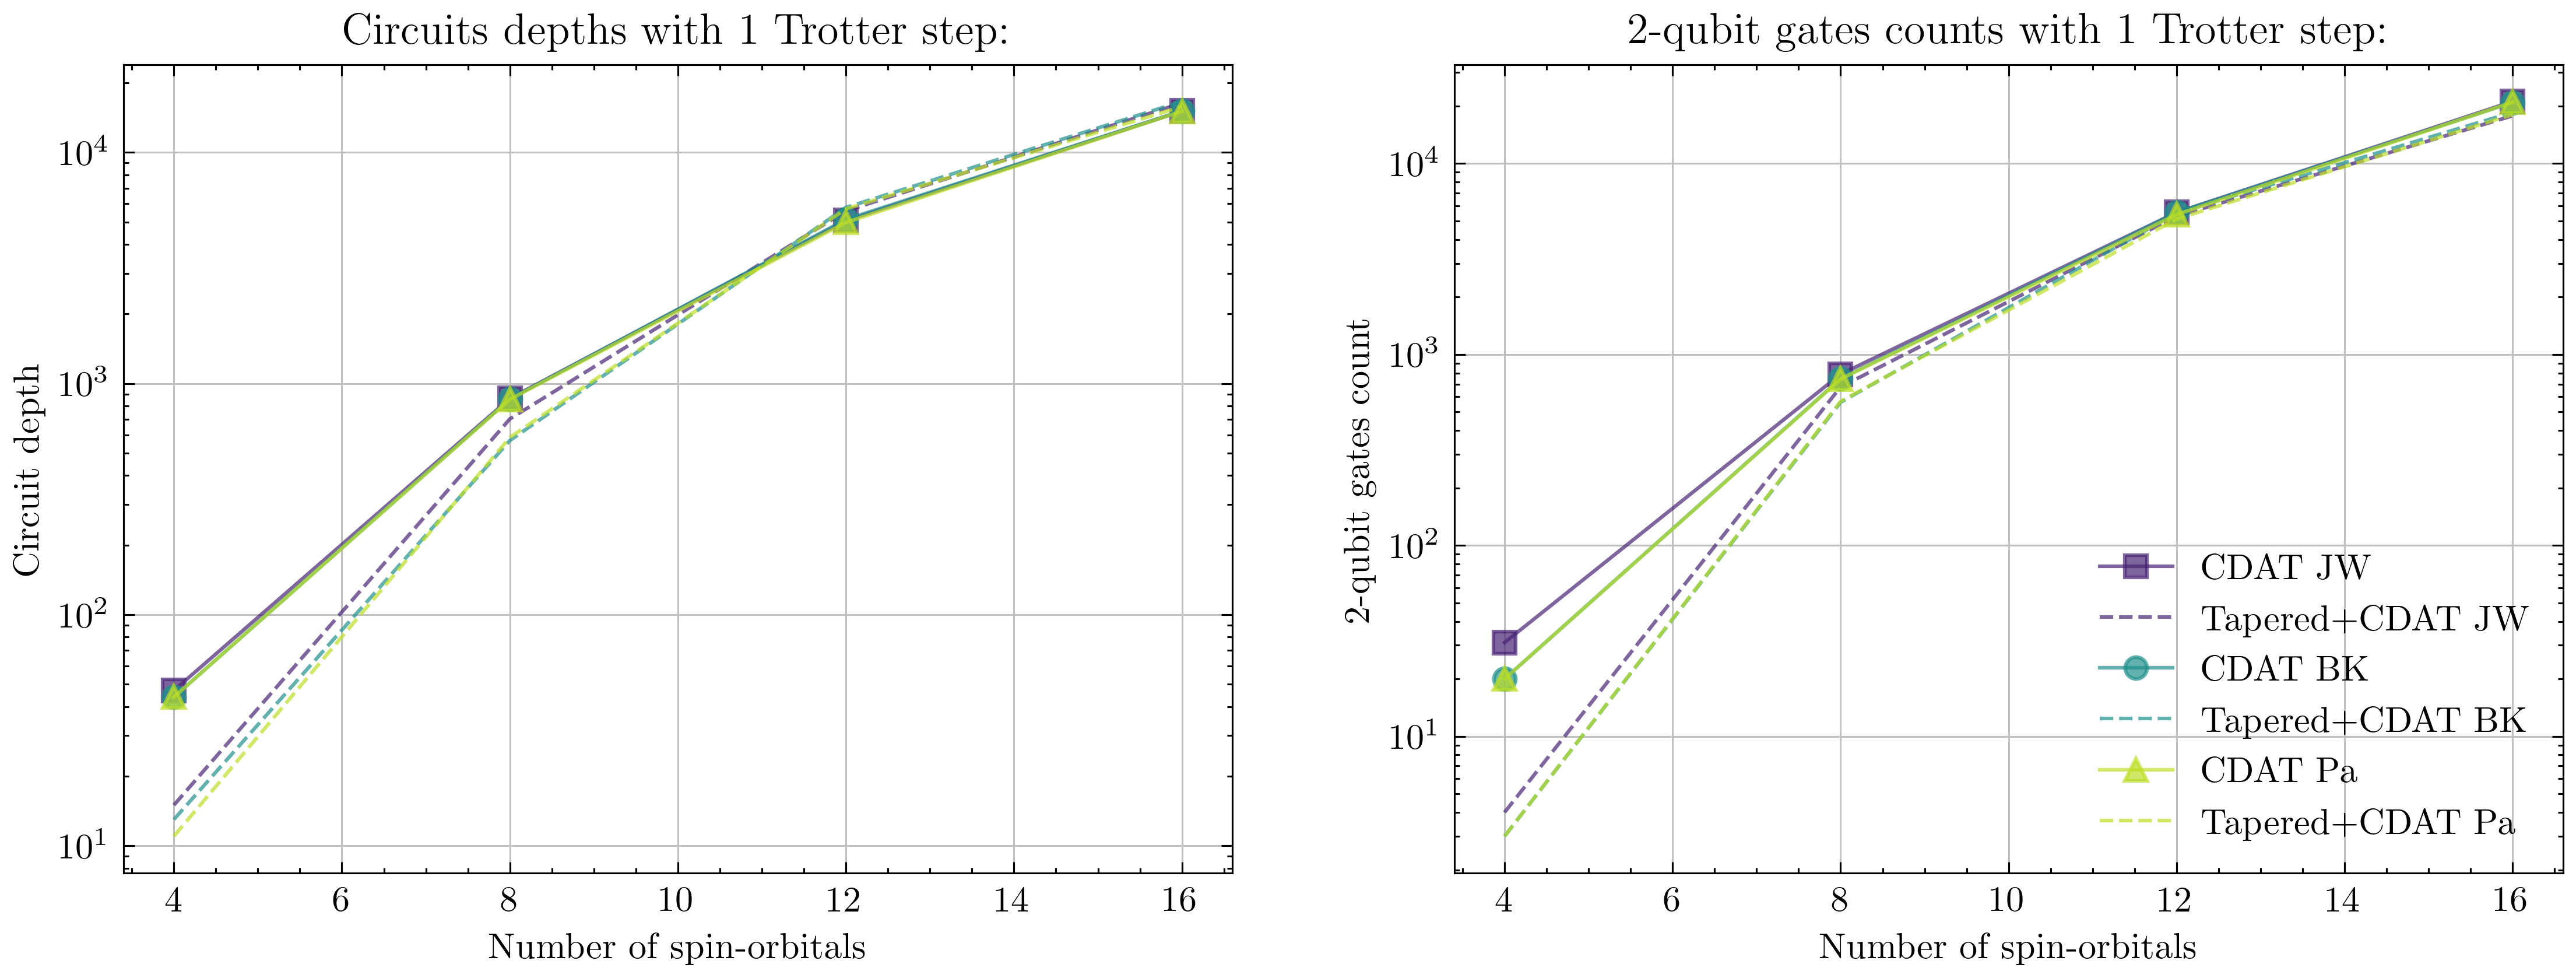}
\caption{\textit{Circuit depths and a number of 2-qubit gates comparison with CDAT applied only and with qubit tapering and CDAT applied for different qubit mappings.}}
\label{fig:CDAT+Tapering circuit reduction results}
\end{figure}

Since qubit tapering did not induce any reduction both applied alone and with CDAT it was not include in the real backend runs or any simulations in this paper.

\newpage
\section{Distribution of Hamiltonian terms' coefficient example}
\label{SI_sec:Ham_term_distribution_example}

A representative example of the distribution of the absolute values of the term's coefficient in 12 qubits example is shown in Figure \ref{fig:ham_terms_coeffs_distr} with the arbitrary coefficients threshold to limit any observable expectation value error to $\epsilon_{d(\langle \hat{A} \rangle )}=2\%$ for the max. time $14$ (a.u.). In this example, only 467 of the default 1807 terms (25.84\%) need to be included for accurate simulation. 
\begin{figure}[h!]
\centering
\includegraphics[width=0.98\linewidth]{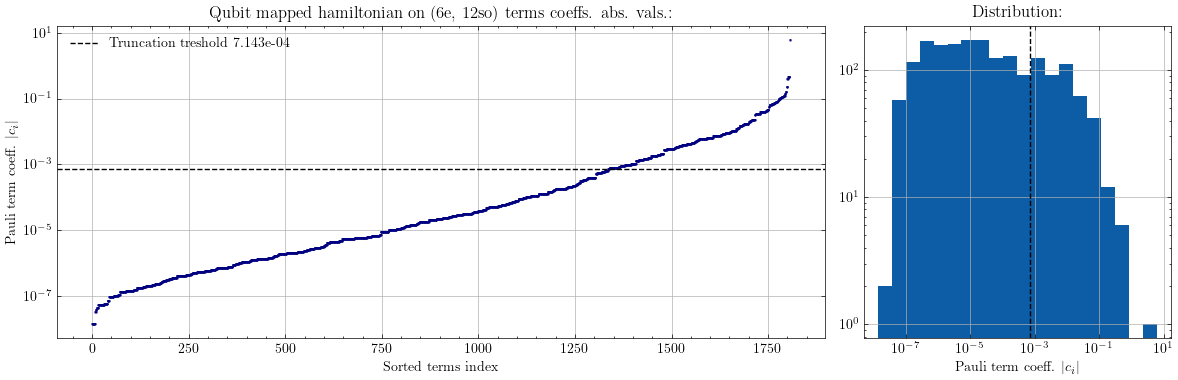}
\caption{\textit{Distribution of the absolute values of the term's coefficient of exemplary molecule with active space (6e, 12so) on 12 qubits with marked coefficients threshold to limit any observable exp. val. error to $\epsilon_{d(\langle \hat{A} \rangle )}=2\%$ for the max. time $14$ (a.u.)}}
\label{fig:ham_terms_coeffs_distr}
\end{figure}
\FloatBarrier

\newpage
\section{Detailed results of QPU runs with middleware}
\label{SI_sec:Haiqu_results}

\begin{figure}
    \centering
    \includegraphics[width=1\linewidth]{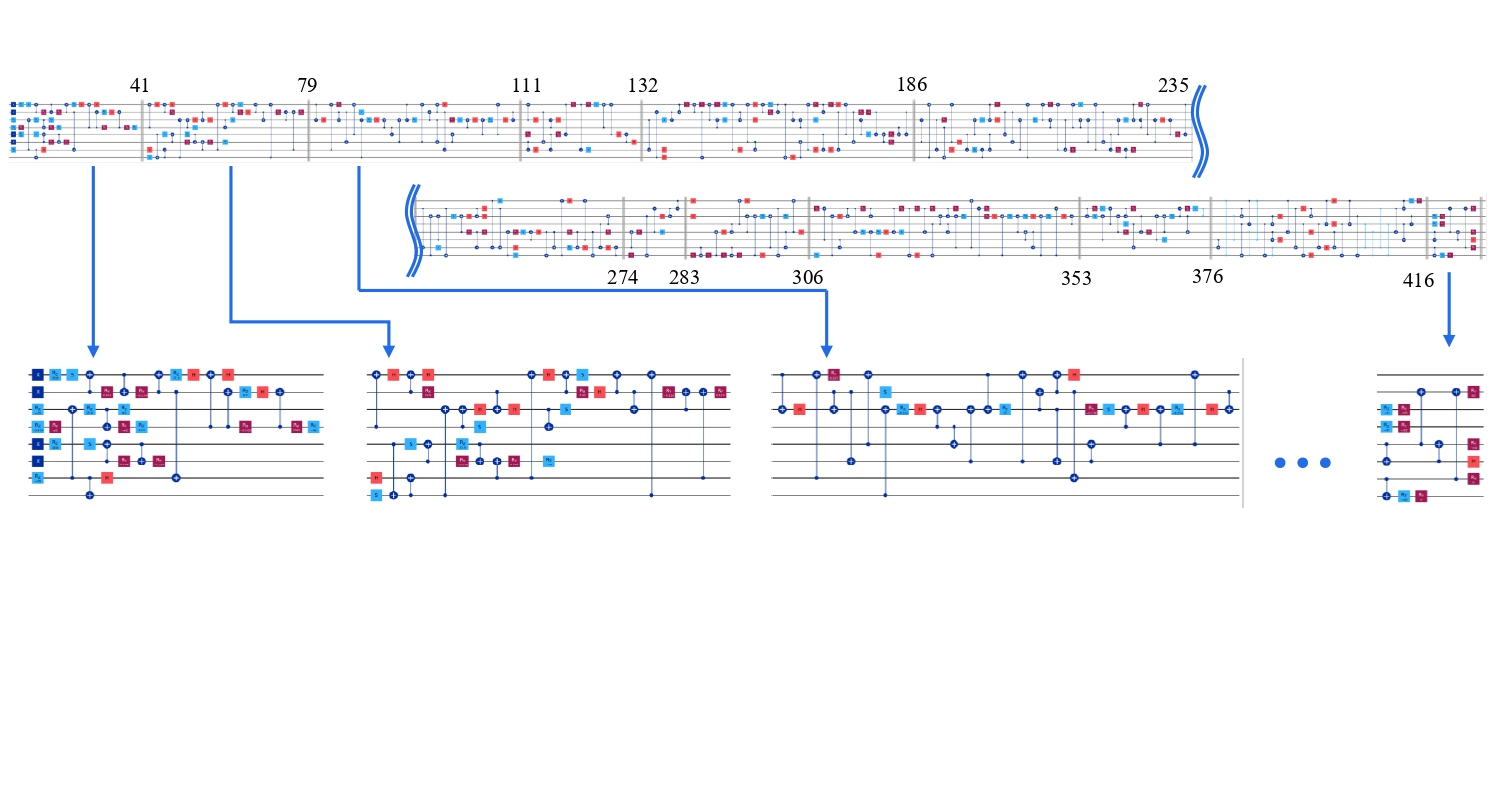}
    \caption{\textit{Decomposition of 8 qubits circuit (similar circuit for the time points 1, 39, 61, 79 and 100) into 13 blocks of size from 9 to 55 gates before the transpilation to device. Numbers indicate the gate count at which barriers are inserted. For time points 61 and 79 we execute circuit combining OE with Operator Backpropagation technique which post processes the second part of the circuit indicated with blue lines.}}
    \label{fig:haiqu_circuit_decomposition}
\end{figure}
\FloatBarrier

In this section, all time steps are shown in atomic units, and the (a.u.) notation is omitted for readability.  

The partitioning strategy within Optimized Execution (OE) is based on multiple variables including circuit structure, layout mapping, sub-block entanglement, and fidelity of its execution on a noisy QPU. In the case of the quantum circuits used for the energy calculation at time steps 1, 39, 61, 79 and 100, the full circuit consisting of 431 gates is partitioned into $N_{blocks}=13$ sub-blocks, as can be seen in Figure \ref{fig:haiqu_circuit_decomposition}. Here, the barriers are added at the depths of 41, 79, 111, 132, 186, 235, 274, 283, 306, 353, 376, and 416. This results in sub-circuits of variable size: from 9 to 55 gates before transpilation to the device. The largest sub-circuit that was run on QPU (after transpilation on IBM Marrakesh architecture) had a depth of 216 and 113 2-qubit gates. After extension with additional quantum gates required by the OE process, the biggest single quantum circuit executed had a depth of 371, and contained 216 2-qubit gates. 

With the OE, the execution of the full circuit on a QPU is performed as $N_{sampling} \times n_{blocks}$ QPU executions of the modified sub-block circuits, with an overhead of $N_{sampling}$ related to sampling the initial state and internal circuit structure, related to specifics of the method. For the problem circuits at hand $N_{sampling} = 600$. Each execution includes the application of custom noise mitigation and suppression pipeline involving dynamical decoupling, Pauli twirling, and readout error mitigation. With $N_{twirls}=8$ twirled circuit copies this sums up to $4800$ circuit executions per sub-block, however, we keep the overall shot budget for a twirled set of $8$ circuits $N_{shots}=10000$. We test our approach on noisy IBM devices using the Heron architecture - the actual IBM Marrakesh QPU, and the IBM FakeTorino simulator, which provides the layout and a high-fidelity noise model of a Heron architecture. 

Given the block nature of the method, we can reconstruct the state at each intermediate barrier. In Figure \ref{fig:haiqu_intermidiate_distribution} a) we plot the intermediate fidelities at different steps for the distributions sampled from the noisy devices with and without Haiqu’s OE approach against the ideal simulation (which is still possible at this qubit scale). We observe that the method performs qualitatively similarly on both real and simulated QPU, resulting in fidelity values significantly higher than the direct execution of the circuit. In Figure \ref{fig:haiqu_intermidiate_distribution} b) we compare the sampled bit-strings distribution for the intermediate state at gate $111$ obtained on the IBM Marrakesh QPU with our method to the one obtained from executing on an ideal simulator. Based on this observation and to save constrained quantum resources, for error bars estimation, we run repeated executions on IBM's FakeTorino simulator. 

Due to the limited hardware QPU accessibility and overhead of the method, to reconstruct the state at the end of the full circuit, we performed part of the execution batches on the actual IBM Marrakesh QPU while some of the intermediate blocks are executed on noisy IBM FakeTorino simulator. The reported last step fidelity and energy values estimation at time steps 1, 39, and 100 are obtained using such a combined approach. For time steps 61 and 79 as a proof of principle we combine the approach with Operator Backpropagation (OB)\cite{Fuller2025} technique allowing to classically process the last part of gates in the circuit. To this end, for time steps 61 and 79 the last part of the circuit indicated by curved blue dividers in Figure \ref{fig:haiqu_circuit_decomposition} is processed by OB. Here the application of OB is motivated due to significant generation of entanglement in the latter steps of the circuit at these particular time steps comparable to high entanglement generated by random Quantum Volume circuit of similar size (see Figure \ref{fig:haiqu_intermidiate_entanglement}), which limits the applicability of OE on the current generation of devices as highly entangled states are more susceptible to noise. The initial observable was backpropagated with allowed approximation error of 0.001 per layer with unlimited number of qubit-wise commuting groups, which in practice corresponded to exact backpropagation.

\FloatBarrier

\vspace{\baselineskip}
\begin{minipage}{\linewidth}
    \captionsetup{type=figure} % -- This line added
    % \centering
    \subcaptionbox{}{\includegraphics[width=1\linewidth]{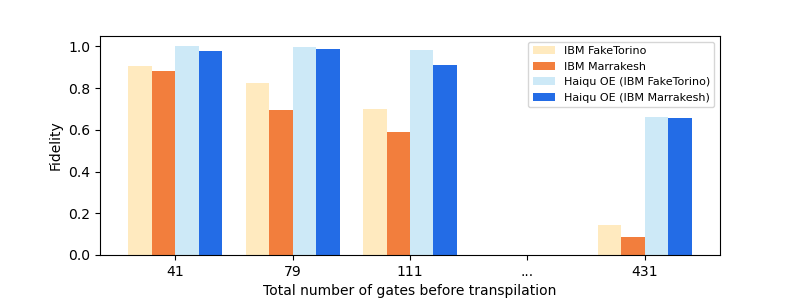}}
    \quad
    \subcaptionbox{}{\includegraphics[width=1\linewidth]{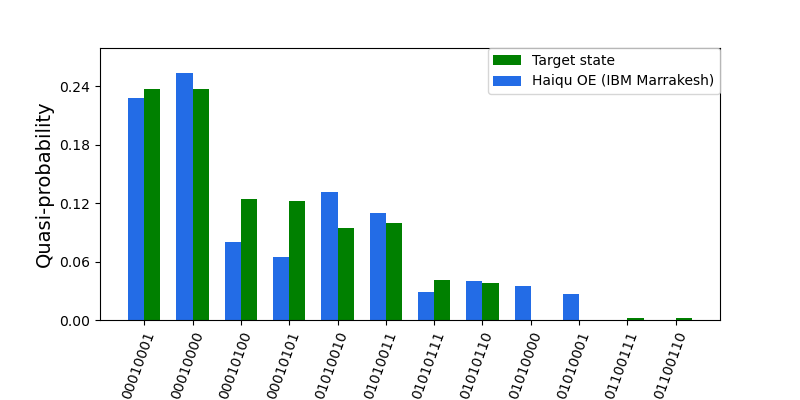}}
    \caption{\textit{(a) Comparison of the fidelity of the 8 qubit circuit at time step 100. On the x-axis, the total number of gates before transpilation executed with Haiqu OE is shown, compared to executing the circuit up to the same point with the default setting on QPU (optimization\_level=3, dynamical decoupling). (b) The intermediate quasi-probability distributions of the target state at gate number 111 compared to that, measured on IBM Marrakesh using Haiqu OE}}
    \label{fig:haiqu_intermidiate_distribution}
\end{minipage}

\vspace{\baselineskip}
\begin{minipage}{\linewidth}
    \captionsetup{type=figure} % -- This line added
    % \centering
    \subcaptionbox{}{\includegraphics[width=0.48\linewidth]{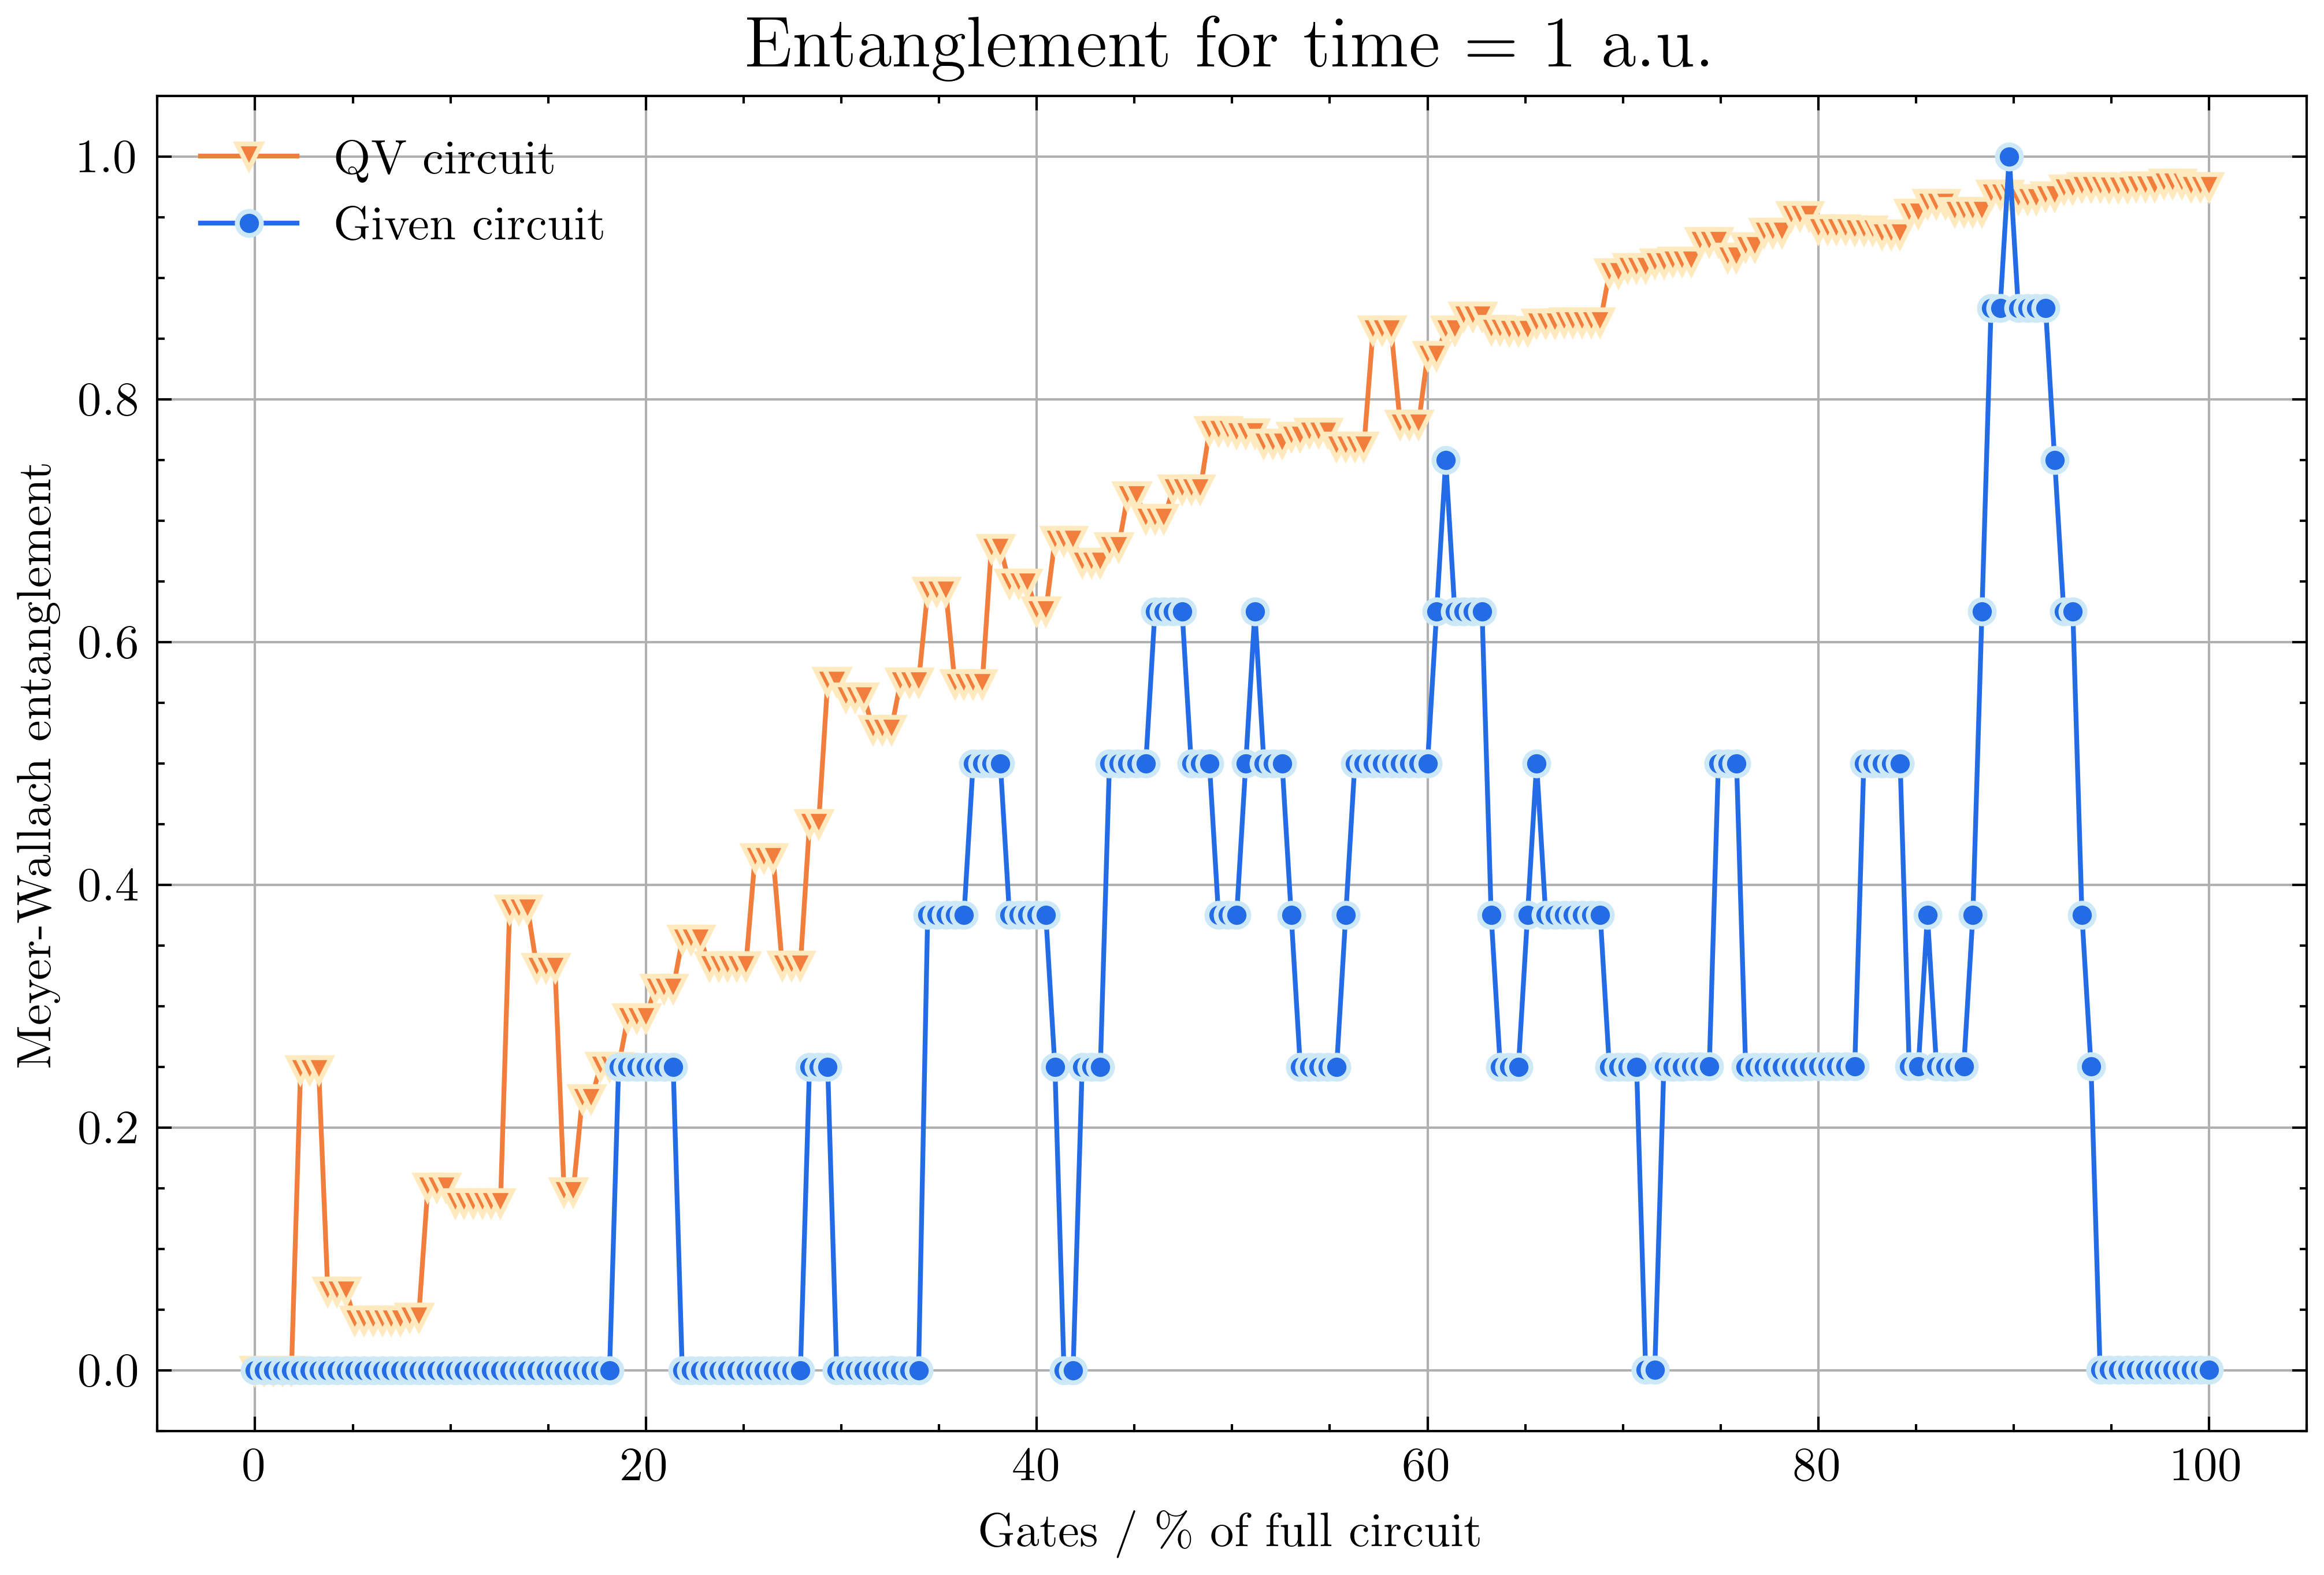}}
    \quad
    \subcaptionbox{}{\includegraphics[width=0.48\linewidth]{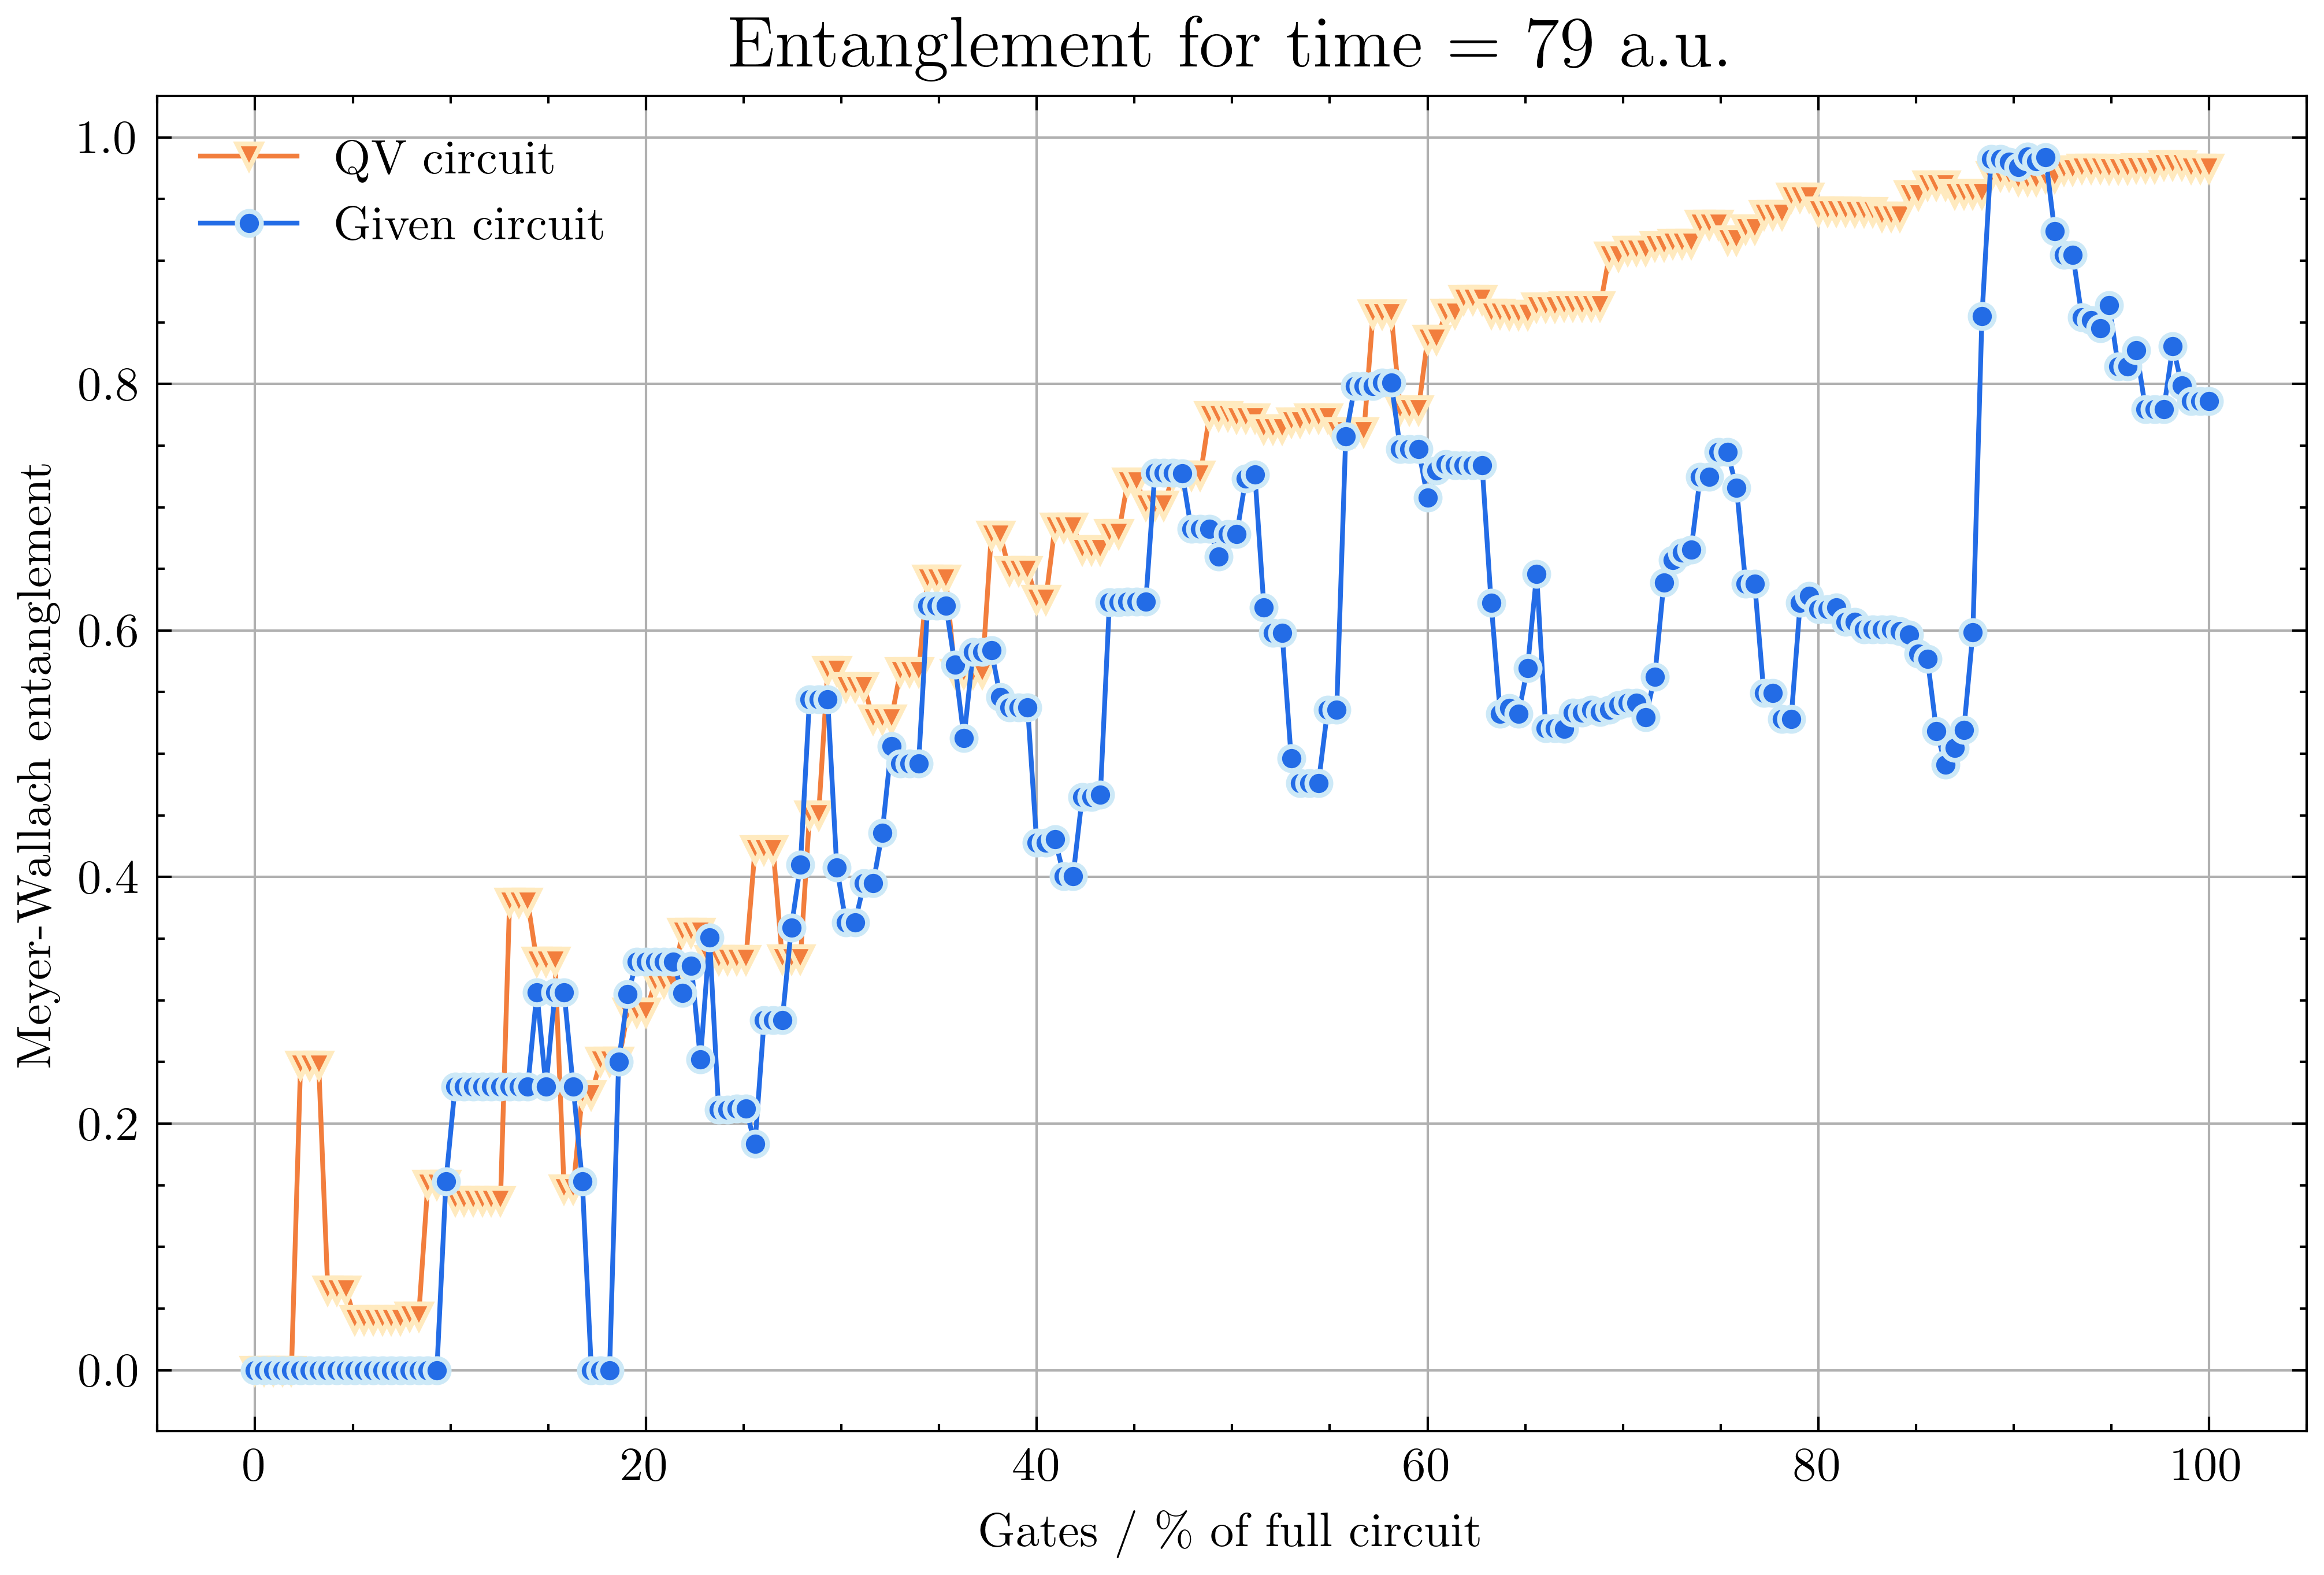}}
    \caption{\textit{Comparison of entanglement growth in the 8 qubit circuit at time steps 1 and 79 through Meyer-Wallach entanglement\cite{Brennen2003}. For intermediate time step 79 entanglement generated by evolution circuit (blue curve) quickly saturates to values comparable or higher than average random Quantum Volume circuit generates (orange curve). As the maximal value of entanglement is located in the end of the circuit, we use Operator Backpropagation technique which allows to execute those gates in a post-processing procedure. }}
    \label{fig:haiqu_intermidiate_entanglement}
\end{minipage}

\renewcommand{\bibsection}{\section*{References}}
\bibliography{supplementary_information}
\bibliographystyle{naturemag}

\end{document}
